# Supplementary material for: Toward end-to-end quantum simulation for protein dynamics
Source: arXiv:2411.03972 source file (2025-04-16)
Supplement: Supplementary file 1 [file supplement.pdf]

# Supplemental materials:
# Toward end-to-end quantum simulation for protein dynamics

Zhenning Liu[1,2], Xiantao Li[3], Chunhao Wang[4], Jin-Peng Liu[5,6,*]

[1] Joint Center for Quantum Information and Computer Science, University of Maryland

[2] Department of Computer Science, University of Maryland

[3] Department of Mathematics, Pennsylvania State University

[4] Department of Computer Science and Engineering, Pennsylvania State University

[5] Yau Mathematical Sciences Center, Tsinghua University

[6] Beijing Institute of Mathematical Sciences and Applications

## Contents

**S1 Preliminaries** 3

S1.1 Notations . . . 3

S1.2 Access models and block-encoding . . . 3

S1.3 QROM and QRAM . . . 5

**S2 Some overview of specific NMA models** 6

S2.1 Normal Modes of All-atom Models . . . 7

S2.2 Network models . . . 8

S2.2.1 Gaussian network model . . . 8

S2.2.2 Anisotropic network model . . . 9

S2.2.3 Network Models with Distance-Dependent Force Constants . . . 9

S2.2.4 All-atom normal mode analysis . . . 9

S2.3 Normal mode dynamics with external effects . . . 10

S2.4 Steered Protein Dynamics . . . 10

**S3 Hierarchical coarse-graining** 11

**S4 QROM based on direct quantization of classical ROM** 12

S4.1 1-of-$N$ decoder . . . 13

S4.2 Hard-coded data loader . . . 13

S4.3 State-based data loader . . . 13

*liujinpeng@tsinghua.edu.cn

**S5 Initial state preparation theorems** **15**
S5.1 The joint state preparation lemma . . . . . 15
S5.2 Proof of Theorem 1 . . . . . 16
S5.3 Quantum mean estimation . . . . . 17
S5.4 Proof of Lemma 2 . . . . . 18
S5.5 Completing the quantized rejection sampling procedure . . . . . 19

**S6 Matrix loading with efficient modification** **20**

**S7 Simulating protein dynamics on quantum computers** **22**
S7.1 Hamiltonian Simulation . . . . . 22
S7.2 LCHS Method for steered protein dynamics . . . . . 24
S7.3 Quantum Linear ODE Solver for the dense outputs . . . . . 25
S7.4 Quantum algorithms for simulating Langevin dynamics . . . . . 27

**S8 Computing properties of proteins** **29**
S8.1 Kinetic and potential energy . . . . . 29
S8.2 Low vibration modes . . . . . 31
S8.3 Density of States and Chebyshev moments . . . . . 33
S8.4 Correlation and root mean square of displacement . . . . . 35
S8.5 Molecular dynamic control . . . . . 36

**S9 Open Problems** **37**

# S1 Preliminaries

## S1.1 Notations

Let $u = (u_0, u_1, \cdots, u_{N-1})^T$ be an $N$-dimensional (possibly unnormalized) column vector. We use $u^*$ to denote its conjugate transpose, $\|u\|$ to denote its vector 2-norm, and $\|u\|_1$ to denote its vector 1-norm. The notation $|u\rangle$ represents a (pure) quantum state that is the normalized vector under 2-norm

$$|u\rangle = u/\|u\|. \tag{S1.1}$$

For quantum states, we follow the standard bra-ket notation where $\langle u|$ denotes the conjugate transpose of $|u\rangle$ and $\langle u|v\rangle$ denotes the inner product between $|u\rangle$ and $|v\rangle$.

Let $A$ be an $N$-by-$N$ matrix. We use $A^\dagger$ to denote its conjugate transpose, *i.e.*, the adjoint operator of $A$. The norm $\|A\|$ without subscript represents the spectral norm, *i.e.*, the matrix 2-norm

$$\|A\| = \sup_{u \neq 0} \|Au\|/\|u\|. \tag{S1.2}$$

The norm $\|A\|_1$ with subscript 1 is the Schatten 1-norm

$$\|A\|_1 = \mathrm{Tr}\left(\sqrt{A^\dagger A}\right). \tag{S1.3}$$

The trace distance between two matrices $A$ and $B$ is defined to be $\frac{1}{2}\|A-B\|_1$, and the trace distance between two pure states $|u\rangle$ and $|v\rangle$ is the trace distance between the corresponding density matrices $|u\rangle\langle u|$ and $|v\rangle\langle v|$.

Let two functions $f, g\colon \mathbb{R}_{>0} \to \mathbb{R}_{>0}$ represent some complexity scalings. We write $f = \mathcal{O}(g)$ if there exists a constant $C > 0$, independent of the arguments of $f$ and $g$, such that $f(x) \leq Cg(x)$ for all sufficiently large $x$. $f = \Omega(g)$ if $g = \mathcal{O}(f)$. $f = \Theta(g)$ if $f = \mathcal{O}(g)$ and $f = \Omega(g)$. $f = \widetilde{\mathcal{O}}(g)$ if $f = \mathcal{O}(g \operatorname{poly}\log(g))$.

## S1.2 Access models and block-encoding

We define the matrix and state preparation oracle access that is commonly used in quantum algorithms.

**Definition S1.1** (Matrix access)**.** Suppose $A$ can be accessed through the following oracle

$$O_r|i,k\rangle = |i, r_{ik}\rangle, \tag{S1.4}$$

$$O_c|i,k\rangle = |i, c_{ik}\rangle, \tag{S1.5}$$

$$O_a|i,j\rangle|0_b\rangle = |i,j\rangle|A(i,j)\rangle, \tag{S1.6}$$

where $r_{ij}$ (resp. $c_{ij}$) are the $j$-th nonzero entry in the $i$-th row (resp. column), and $A(i,j)$ is the binary representation of the $(i,j)$ matrix entry of $A$.

**Definition S1.2** (State preparation)**.** Let $y$ be a $2^n$-dimensional vector and $\|y\|_1 \leq \beta$. Then a unitary $U_I$ is a $(\beta, n, 0)$-state-preparation oracle, if $U_I|0\rangle = \frac{1}{\beta}\sum_{j=0}^{2^n-1} y_j |j\rangle$.

Block-encoding is a powerful technique to represent arbitrary matrices with unitary matrices. For a possibly non-unitary matrix $A$ and a parameter $\alpha \geq \|A\|$, the intuitive idea of block-encoding is to construct a unitary $U$ with higher dimension such that $A$ appears in its upper-left block,

$$U = \begin{pmatrix} A/\alpha & * \\ * & * \end{pmatrix}. \tag{S1.7}$$

More results about the block-encoding refer to [29].

**Definition S1.3** (Block-encoding)**.** Suppose $A$ is a $2^n$-dimensional matrix such that $\|A\| \leq \alpha$. Then a $2^{n+a}$-dimensional unitary matrix $U$ is an $(\alpha, a, \epsilon)$-block-encoding of $A$, if

$$\|A - \alpha(\langle 0|_a \otimes I)U(|0\rangle_a \otimes I)\| \leq \epsilon. \tag{S1.8}$$

Block-encoding allows us to encode a general matrix on quantum computers and then perform matrix operations, including summation, multiplication, inverse, and polynomial transformation. Here we mostly follow [29] again and briefly summarize several properties that will be used in our work.

**Definition S1.4** (State preparation pair)**.** Let $y$ be a $2^n$-dimensional vector and $\|y\|_1 \leq \beta$. Then a pair of unitaries $(U_{IL}, U_{IR})$ is a $(\beta, n, 0)$-state-preparation-pair, if $U_{IL}|0\rangle = \sum_{j=0}^{2^n-1} c_j |j\rangle$, $U_{IR}|0\rangle = \sum_{j=0}^{2^n-1} d_j |j\rangle$ and $\beta c_j^* d_j = y_j$ for any $0 \leq j \leq 2^n - 1$.

**Lemma S1.5** (Linear combination of block-encodings [29, Lemma 52])**.** *Let $A = \sum_{j=0}^{2^k-1} y_j A_j$ be a $2^n$-dimensional matrix. Suppose that $(U_{IL}, U_{IR})$ is a $(\beta, k, 0)$-state-preparation-pair of $y$, and $W = \sum_{j=0}^{2^k-1} |j\rangle\langle j| \otimes U_j$ is a $2^{n+a+k}$-dimensional unitary matrix such that $U_j$ is an $(\alpha, a, \epsilon)$-block-encoding of $A_j$. Then $(U_{IL}^\dagger \otimes I_a \otimes I_n)W(U_{IR} \otimes I_a \otimes I_n)$ is an $(\alpha\beta, a+k, \alpha\beta\epsilon)$-block-encoding of $A$, with a single use of $W, U_{IL}^\dagger$ and $U_{IR}$.*

**Lemma S1.6** (Multiplication of block-encodings [29, Lemma 53])**.** *Let $A, B$ be $2^n$-dimensional matrices, $U_A$ be an $(\alpha, a, \delta)$-block-encoding of $A$, and $U_B$ be a $(\beta, b, \epsilon)$-block-encoding of $B$. Then $(I_b \otimes U_A)(I_a \otimes U_B)$ is an $(\alpha\beta, a+b, \alpha\epsilon + \beta\delta)$-block-encoding of $AB$, with a single use of $U_A$ and $U_B$.*

**Lemma S1.7** (Inverse of a block-encoding [58, Appendix B])**.** *Suppose $A$ is a $2^n$-dimensional invertible Hermitian matrix such that all the eigenvalues are within $[-1, -\delta] \cup [\delta, 1]$, and $U_A$ is a $(1, a, 0)$-block-encoding of $A$. Then a $(4/(3\delta), a+1, \epsilon)$-block-encoding of $A^{-1}$ can be constructed, using $\mathcal{O}((1/\delta)\log(1/(\delta\epsilon)))$ queries to $U_A$ and its inverse.*

**Lemma S1.8** (Polynomial of a block-encoding [29, Theorem 56])**.** *Let $A$ be a $2^n$-dimensional Hermitian matrix, and $U_A$ is an $(\alpha, a, \epsilon)$-block-encoding of $A$. If $P(x)$ is a degree-$d$ real polynomial such that $|P(x)| \leq 1/2$ for all $x \in [-1, 1]$, then a $(1, a+2, 4d\sqrt{\epsilon/\alpha})$-block-encoding of $P(A/\alpha)$ can be constructed using $d$ applications of $U_A$ and $U_A^\dagger$, a single application of controlled $U$ and $\mathcal{O}((a+1)d)$ additional one- and two-qubit gates.*

We use the following technical tool to estimate the expectation of block-encoded observables.

**Lemma S1.9** ([54]). *Let $O$ be an observable whose block-encoding has normalizing constant $\alpha$ and construction cost $Q$. If a purification of a state $\rho$ can be prepared with cost $R$, then for every $\epsilon, \delta > 0$, there exists a quantum algorithm that products an estimate $\xi$ of $\mathrm{Tr}(\rho O)$ such that*

$$|\xi - \mathrm{Tr}(\rho O)| \leq \epsilon$$

*with probability at least $1 - \delta$. This algorithm has gate complexity $\mathcal{O}((R + Q)\frac{\alpha}{\epsilon}\log(1/\delta))$.*

## S1.3 QROM and QRAM

In this paper, we use Quantum Read-Only Memory (QROM) [9, 53] (also known as Quantum Random-Access Classical Memory, QRACM, as a read-only version of QRAM) as a time-efficient method of loading classical data into the quantum algorithm. QROMs can coherently provide the data corresponding to an address according to a classical dictionary. For instance, if a dictionary is given such that for every index $i \in \{1, 2, \ldots, N\}$ the data is an arbitrary $v_i \in \{1, 2, \ldots, M\}$, then a QROM of this dictionary implements the following unitary:

$$\sum_i \alpha_i |i\rangle |0\rangle \mapsto \sum_i \alpha_i |i\rangle |v_i\rangle . \tag{S1.9}$$

Many proposals for QROM or QRAM are available in the literature and they are either *passive* or *active* [37]. Passive QROMs can realize the data loading operation just like a single quantum gate without sophisticated error correction, such as [30], but are considered impractical because an exponentially low error rate is required [37]. Instead, we focus on active QROM/QRAMs that can be constructed explicitly by quantum circuits of $\tilde{\mathcal{O}}(N)$ gates but in $\mathcal{O}(\log N)$ depth, when the amount of data stored is $\mathcal{O}(N)$. We notice that we aim at achieving exponential speedup in terms of $N$, but QROM's gate complexity scales linearly in $N$. We claim that this is an unavoidable cost, as shown in Theorem S1.10 also proved in [37]. We instead focus on achieving an exponential speedup in time complexity in this paper.

**Theorem S1.10** (Gate complexity lower bound of data loading). *Suppose there is a unitary $U$ such that for all $\sum_{i=1}^{N} \alpha_i |i\rangle$ with $\sum_{i=1}^{N} |\alpha_i|^2 = 1$, and for any ancilla register in state $|R\rangle$,*

$$U \left[ |R\rangle \otimes \sum_{i=1}^{N} \alpha_i |i\rangle |0\rangle \right] = |R\rangle \otimes \sum_{i=1}^{N} \alpha_i |i\rangle |d_i\rangle$$

*where each $d_i$ is an arbitrary $m$-bit binary string. Then the quantum circuit implementing $U$ must have at least $\mathcal{O}(Nm)$ elementary gates.*

*Proof.* Since all $d_i$ strings are arbitrary, we can prove the result using the counting argument. The classical data to be loaded can be considered as a dictionary $\{(i, d_i) | i \in [N]\}$, which contains $Nm$ bits in total. The total number of possible dictionaries is therefore $2^{Nm}$. The unitary $U$ must be able to distinguish between all $2^{Nm}$ possibilities. If $U$ is composed of an elementary gate set in which each gate acts on a constant number of qubits, then the number of gates required to distinguish $2^{Nm}$ cases is $\log(2^{Nm}) = \mathcal{O}(Nm)$. □

Previous results [9, 53, 5] suggested different architectures to implement QROM with different trade-offs between circuit depth and width. In Section S4, we propose a new scheme of QROM by direct quantization of classical Read-Only Memory with logarithmic depth and a width-depth tradeoff feature.

However, as [37] points out, asymptotic advantages of quantum algorithms in time complexity may also be affected by circuit-based active QROM/QRAM. This is because the number of (logical) qubits involved in a QRAM/QROM circuit is at least $\Omega\left(\frac{N}{\log N}\right)$, which requires a significant amount of effort in classical control. Since controlling a logical qubit is difficult, the classical controlling resources required can be considered as $\Omega\left(\frac{N}{\log N}\right)$ parallel processors. When so many processors are used, it is possible that a classical parallel algorithm can solve the same computational problem in a comparable amount of time. However, we argue that as experimental techniques evolve, classical control of qubits will become less challenging such that $\frac{N}{\log N}$ qubits require a comparable amount of control as $\frac{N}{\log N}$ classical bits, much less than $\frac{N}{\log N}$ parallel classical computers. In this case, an exponential speedup in time complexity is a significant improvement over classical computation. For instance, in Ref. [13], an experimental platform based on reconfigurable atom array features collective control of a set of physical qubits composing a logical qubit. Although there is still a significant amount of effort to control each logical qubit, it is hopeful for future devices to use much fewer classical control lines. In such a case, the classical co-processors should not be considered as a large parallel computer. We also notice that [1] if fan-in gates can be implemented in some experimental platforms, then circuit depth for QRAM/QROM can even be reduced to a constant, even though qubit number required still scales linearly in the amount of data.

## S2 Some overview of specific NMA models

Here we give an overview of some of the existing models. All these models can be recast into linear differential equations

$$M\frac{\mathrm{d}^2}{\mathrm{d}t^2}\boldsymbol{u} = -K\boldsymbol{u}. \tag{S2.1}$$

while the matrix $K$ can be modeled differently. Overall, the underlying assumption in NMA is that any given equilibrium system fluctuates about a single well-defined conformation and that the nature of these thermally induced fluctuations can be calculated assuming a simple harmonic form for the potential. In NMA, a protein consists of a collection of nodes, here labeled by $i \in [N] \coloneqq \{1, 2, \ldots, N\}$. Further, we denote the instantaneous position of the $i$-th node by $R_i$ with equilibrium position $R_i^0$. Therefore the dynamics is reflected in the displacement vector $\boldsymbol{u}_i = R_i - R_i^0$. We also denote the relative position between two atoms, $i$ and $j$, by $\boldsymbol{u}_{ij} = R_i - R_j$ with equilibrium values $R_{ij}^0$.

An intuitive interpretation of the NMA model is that every pair of neighboring nodes is connected by a spring with a spring constant given by $K_{i,j}$. Therefore the total potential energy is

given by the following quadratic form,

$$V(\boldsymbol{u}) = \frac{1}{2}\sum_{ij=1}^{N} \boldsymbol{u}_i K_{ij} \boldsymbol{u}_j. \tag{S2.2}$$

Then the equations in (S2.1) follow directly from standard Hamilton or least-action principle.

A solution of (S2.1) has the form $\hat{\boldsymbol{u}}_k(t) = \boldsymbol{a}_k \exp(-i\omega_k t)$, where $a_k$ contains both the amplitude and phase factor, and $\omega_k$ is the frequency. The equation of motion becomes

$$\omega_k^2 M \hat{\boldsymbol{u}}_k = K \hat{\boldsymbol{u}}_k, \tag{S2.3}$$

or a matrix diagonalization form,

$$KU = MU\Lambda, \tag{S2.4}$$

where $U$ collects $\{K\hat{\boldsymbol{u}}_k\}_k$ as its columns and $\Lambda$ collects $\{\omega_k^2\}_k$ as its diagonal elements.

In the energy spectrum, $\omega_k$ corresponds to the vibration frequency and the associated normal mode $\hat{\boldsymbol{u}}_k$ carries energy,

$$V(\boldsymbol{u}) = \frac{1}{2}\hat{\boldsymbol{u}}_k^T K \hat{\boldsymbol{u}}_k = \frac{\omega_k^2}{2}. \tag{S2.5}$$

The vibration frequencies are usually divided into low (or soft) modes, which indicate a less steep gradient along the energy landscape and thus energetically favorable, and high-frequency (or excited) modes, which require much higher thermal energy to reach. Displacements along high-frequency modes are therefore energetically more expensive than those of equal magnitude along low-frequency modes. The vibrational energy is, on average, equally partitioned among all the modes, such that the average amplitude of oscillation along mode $k$ scales with $1/\omega_k^2$. Thus, the molecule experiences the greatest displacement along the lowest frequency, or "slowest", modes. Conceptually, the energy landscape slopes most gently along the slow modes, and these are consequently the most accessible. These modes are also of great interest when seeking to determine the most probable global fluctuations of a molecule. Large eigenvalues, on the other hand, indicate directions of steep energetic ascent, and excursions along these modes will quickly raise the system's energy.

In the following sections, we will give several examples of the stiffness matrix $K$ as well as the matrix structure, which will be important in the preparation of the quantum algorithms. Further generalizations, including the interactions with the solvent and the presence of external forces, will be presented later in Sections S2.3 and S2.4.

## S2.1 Normal Modes of All-atom Models

A normal model model can be directly obtained from MD (S2.1) by a Taylor expansion. Specifically, at an equilibrium configuration $\{R_i^0, i \in [N]\}$, the force on each atom vanishes, i.e., $\nabla V(R_1^0, R_2^0, \cdots, R_N^0) = 0$. Thus a Taylor expansion up to second-order yields,

$$V(R_1, R_2, \cdots, R_N) \approx V(R_1^0, R_2^0, \cdots, R_N^0) + \frac{1}{2}\sum_{i,j=1}^{N} \boldsymbol{u}_i^T K_{i,j} \boldsymbol{u}_j, \tag{S2.6}$$

where $\boldsymbol{u}_i := R_i - R_i^0$ indicates the displacement from the equilibrium position. In addition,

$$K_{i,j} := \nabla^2_{R_i,R_j} V(R_1^0, R_2^0, \cdots, R_N^0), \tag{S2.7}$$

corresponds to the $(i,j)$ block of the Hessian matrix, and it is often referred to as the force constant matrix. The translational symmetry implies that [6],

$$\sum_{j=1}^{N} K_{i,j} = 0. \tag{S2.8}$$

Meanwhile, the approximation (S2.6) is known as a harmonic approximation, which simplifies the equations of motion to a linear ODE system in (S2.1). In other words, the elements of the stiffness matrix $K$ are obtained from the hessian of the interatomic potential $V$ at an equilibrium.

## S2.2 Network models

Another widely used model for normal mode calculations is based on mapping protein structures to a network, where the connectivity is represented by the edges of the network. It has been motivated by the observation that the low modes typically correspond to the cooperative movement of the $C^\alpha$ atoms on the backbone [11], which can be qualitatively described by an elastic network. This idea has been later generalized to incorporate anisotropic motions and networks of all the atoms. Typically, in a network model, one designates a set of nodes that correspond to either the displacement of the $C^\alpha$ atoms or all the atoms in the molecule, with displacement denoted by $\boldsymbol{u} \in \mathbb{R}^M$. The vibration potential is then expressed as,

$$V = \frac{1}{2}\boldsymbol{u}^T \Gamma \boldsymbol{u}. \tag{S2.9}$$

The matrix $\Gamma$ is a symmetric semi-positive definite matrix known as the Kirchhoff or connectivity matrix. The elements in $\Gamma$ can be interpreted as the weights in the network. They are designated empirically, rather than computed from the force field, which drastically simplifies the accessibility of the models. Thus, the variation among different network models comes from the designations of the nodes $\Delta R$ and the specifications of the Kirchhoff matrix.

### S2.2.1 Gaussian network model

The Gaussian network model [10, 32] works directly with the $C^\alpha$ atoms and is built on the assumption that the relative distance between $C^\alpha$ atoms follows a Gaussian distribution. The coupling of the $C^\alpha$ atoms is modelled by a connectivity matrix $\Gamma$, with elements $\Gamma_{ij}$ selected as the Laplacian matrix of inter-residue contacts,

$$\Gamma_{ij} = \begin{cases} -1, & i \neq j,\ R_{ij}^0 \leqslant r_c, \\ 0, & i \neq j,\ R_{ij}^0 > r_c, \\ -\sum_{j,j\neq i} \Gamma_{ij}, & i = j. \end{cases} \tag{S2.10}$$

The parameter $r_c$ is a cut-off radius that identifies neighboring $C^\alpha$ atoms. Meanwhile, the stiffness matrix $K$ is set to $K = \gamma\Gamma$ with $\gamma$ being a force constant uniform for all connected nodes.

### S2.2.2 Anisotropic network model

Implicit in the GNM model is that the displacement of each node is isotropic, in that the components $\Delta X, \Delta Y$, and $\Delta Z$ are independent and identically distributed, given by the distribution of $\Delta R$. The Anisotropic Network Model (ANM) [7] is an extension of GNM to include all three coordinates for each $C^\alpha$ atom, thus accounting for directional movements. In this case, we can write $R_i = [X_i, Y_i, Z_i]$, $R_j = [X_j, Y_j, Z_j]$ be the instantaneous positions of atoms $i$ and $j$. Further, let $R_{ij} = R_i - R_j$ be the relative position, with $d_{ij}$ be the equilibrium distance. In ANM, the Kirchhoff matrix is obtained by assuming that the energy between the two atoms is modeled by a harmonic spring with spring constant $\gamma$,

$$V_{ij} = \frac{\gamma}{2}(\|R_{ij}\| - d_{ij})^2. \tag{S2.11}$$

Therefore, by taking the second-order derivatives, one has,

$$\frac{\partial^2 V_{ij}}{\partial X_i^2} = \frac{\partial^2 V_{ij}}{\partial X_j^2} = \frac{\gamma}{d_{ij}^2}(X_j - X_i)^2, \quad \frac{\partial^2 V_{ij}}{\partial X_i \partial Y_j} = -\frac{\gamma}{d_{ij}^2}(X_j - X_i)(Y_j - Y_i). \tag{S2.12}$$

As a result, the matrix $K$ can be expressed in a block form, $[K_{i,j}]$ with each block being a $3\times 3$ matrix,

$$K_{ij} = \begin{cases} -\frac{\gamma}{d_{ij}^2} R_{ij}^0 (R_{ij}^0)^T, & i \neq j \\ -\sum_{j\neq i} K_{ij}, & i = j. \end{cases} \tag{S2.13}$$

### S2.2.3 Network Models with Distance-Dependent Force Constants

In GNM and ANM, the elastic springs are introduced between atoms within a certain proximity, i.e., when the distance is within a cut-off radius. This can be accomplished by choosing $K_{ij} = 0$, where the distance between the two atoms $d_{ij} > r_c$. Fuglebakk [28] extended this choice by introducing a distance dependence in $K$. For example, in the Harmonic $C^\alpha$ Potential Model (HCA), the force constants are given by

$$K_{ij} = \begin{cases} a_1 d_{ij} - b, & i \neq j,\ d_{ij} \leqslant r_c \\ a_2 d_{ij}^{-6}, & i \neq j,\ d_{ij} > r_c. \end{cases} \tag{S2.14}$$

Here the parameter $r_c$ is set to be 0.4 nm to separate interactions between $C_\alpha$ atoms adjacent in sequence from the other interactions. Long-range interactions are proportional to an inverse power of six of the equilibrium distance between the interacting modes. The parameters $a_1$, $a_2$, $b$ are chosen by fitting an all-atom normal mode calculation for crambin.

Another important approach is the parameter-free anisotropic network model (pfANM), which defines force constants by the inverse-square of the equilibrium distance between the interacting modes. A similar example is the Realistic Extension Algorithm via Covariance Hessian (REACH), which offers a refined treatment for the force constants to incorporate the backbone interactions.

### S2.2.4 All-atom normal mode analysis

As illustrated in Section S2.1, the normal mode analysis can be derived from the full atomistic description with $K$ corresponding to the hessian of the potential energy. In practice, however, this

can be quite a cumbersome effort. Hu et al [34] proposed to consider atoms as point masses and model the bonding between atoms as elastic springs, thus empirically mapping the atomistic model to an elastic network. The total elastic energy is also a quadratic form Eq. (S2.9) and the stiffness parameters in [34] are chosen based on the interatomic distance,

$$K_{ij} = \begin{cases} C_{\text{nonbonded}}, & d_{ij} \leqslant l_1 \\ C_{\text{nonbonded}} \cdot \exp\{(-(d_{ij} - l_1))\}, & l_1 \leqslant d_{ij} \leqslant l_2 \\ 0, & d_{ij} \geqslant l_2. \end{cases} \tag{S2.15}$$

Here $d_{ij}$ is the distance between two atoms: $d_{ij} = \left\| R_i^0 - R_j^0 \right\|$, $C_{\text{bonded}} = 7 \times 10^5$ dyne/cm is a nominal spring constant generally assigned to a single bond, and $C_{\text{nonbonded}} = 6 \times 10^3$ dyne/cm is for non-bonded interactions, $l_1$ and $l_2$ are the lower and upper cutoff values, under the consideration of the maximum range of van der Waals interaction, e.g., $l_1 = 2\mathring{A}$, and upper-bound cutoff distance $l_2 = 8\mathring{A}$. This model is later extended [35], where the stiffness matrix $(k_{i,j})$ is determined based on the chemical connectivity and atomic interaction, rather than the cutoff-distance.

## S2.3 Normal mode dynamics with external effects

Solvent molecules, typically water, interact with the protein's surface through hydrogen bonding and hydrophobic interactions, which may directly impact the protein's conformation. A simple way to model the effect of solvent molecules is by Langevin dynamics, which after the harmonic approximation of the inter-molecular forces, leads to the linear stochastic differential equation

$$M \frac{\mathrm{d}^2 \boldsymbol{u}}{\mathrm{d}t^2} = -\gamma \frac{\mathrm{d}\boldsymbol{u}}{\mathrm{d}t} - K\boldsymbol{u} + \xi(t). \tag{S2.16}$$

Here $\gamma$ is a friction coefficient and it provides velocity-dependent damping. Meanwhile, the white noise $\xi$ accounts for thermal energy transferred to the molecule from the solvent. The elements of this vector obey the properties

$$\mathbb{E}[\xi_i(t)] = 0 \tag{S2.17}$$

and the fluctuation-dissipation theorem,

$$\mathbb{E}[\xi_i(t)\xi_j(t')] = 2\gamma k_B T \delta_{ij} \delta(t - t'). \tag{S2.18}$$

## S2.4 Steered Protein Dynamics

Another simple extension is the normal mode dynamics under a mechanical force,

$$M \frac{\mathrm{d}^2 \boldsymbol{u}}{\mathrm{d}t^2} = -K\boldsymbol{u} + \boldsymbol{f}(t), \tag{S2.19}$$

where $\boldsymbol{f}(t)$ can be regarded as a mechanical load.

This idea has been pursued in the steered MD approach [36], where the forces are used to speed up the folding process. Similarly, Arkun and Gur considered the driven dynamics (S2.19) in an optimal control framework, where $\boldsymbol{f}(t)$ involves control variables that are determined by minimizing a cost function.

# S3 Hierarchical coarse-graining

Coarse-grained models are commonly employed to describe the structure and dynamics of large molecular systems.

We build a hierarchical network model based on Markov stochastics [25, 16, 17]: step (i) map the structure to its optimal reduced level representation. This step may involve several intermediate levels of resolution; step (ii) performs structural analysis (e.g. ENM, GNM) at a coarse-grained scale; and step (iii) reconstructs the detailed structure-dynamics. The communication/coupling of residues at a given level is assumed to obey a Markov process controlled by atom-atom contact topology. The steps (i) and (iii) are achieved by two operators, $R$ for model reduction, and $K$ for model reconstruction. $R$ and $K$ ensure that similar stochastic characteristics are retained between successive levels of the hierarchy.

We model each protein as a weighted,undirected graph $G = (V, E)$, with residues $V = \{v_1, \ldots, v_n\}$ and interactions $E = \{e_{ij}\}$. The set of all pairwise interactions is described by a non-negative, symmetric affinity matrix $A$, with element $a_{ij} = a_{ji}$. The element $a_{ij} = N_{ij}$ is the total number of atom-atom contacts made between residues $v_i, v_j$ and within a cutoff distance $r_c = 4.5\mathring{A}$. The self-similar contact $a_{ii}$ is similarly defined, but all bonded pairs are excluded. An alternative definition is $a_{ij} = N_{ij}/\sqrt{N_i N_j}$, where $N_i$ is the total number of atoms in the residue $v_i$.

This representation takes into account the difference in the size of amino acids, and captures to a first approximation the strong (weak) interactions expected to arise between residue pairs with a large (small) number of atom-atom contacts.

The degree of the residue $v_i$ is defined as $d_i = \sum_{j=1}^{n} a_{ij}$. We define $D = \mathrm{diag}(d_1, \ldots, d_n)$.

We define a Markov transition matrix on the protein graph as $M = AD^{-1}$, with element $m_{ij} = a_{ij} d_i^{-1}$ as the probability of transition from residue $v_i$ to $v_j$. The Markov chain has a unique stationary distribution $\pi$ with $\pi_i = d_i/(\sum_{j=1}^{n} d_j)$.

The objective in designing a network hierarchy is to map the Markov process operating at the highest resolution onto successively lower resolution network models, while maintaining its stochastic characteristics. Using the $n \times n$ Markov transition matrix $M$ and stationary distribution $\pi$, we build a $m \times m$ coarse-scale Markov transition matrix $\widetilde{M}$ ($m \ll n$) and its stationary distribution $\delta$. To build a hierarchy of intermediate resolution networks, we devise two operators at each level of the hierarchy: $R$ for model reduction, and $K$ for model reconstruction.

We express $\pi$ as a mixture of latent distributions

$$\pi = K\delta, \tag{S3.1}$$

where $\delta$ is a unknown stationary distribution in the reduced space and $K = \{K_{ij}\}$ is an $n \times m$ non-negative kernel matrix, acting as an expansion operator.

We derive a maximum likelihood approximation for $\delta$ using an Expectation-Maximization (EM) algorithm. We minimize the Kullback-Liebler divergence subject to the constraint $\sum_{j=1}^{m} \delta_j = 1$

ensured by the Lagrange multiplier $\lambda$

$$E = -\sum_{i=1}^{n} \pi_i \ln \sum_{j=1}^{m} K_{ij}\delta_j + \lambda(\sum_{j=1}^{m} \delta_j - 1). \tag{S3.2}$$

Taking the derivative of $E$ with respect to $\delta_j$ to be zero, we obtain

$$\sum_{i=1}^{n} \frac{\pi_i K_{ij}\delta_j}{\sum_{k=1}^{m} K_{ik}\delta_k} = \lambda \delta_j. \tag{S3.3}$$

We can define ownership of the node $i$ in the high resolution to the kernel $j$ in the low resolution as

$$R_{ij} = \frac{K_{ij}\delta_j}{\sum_{k=1}^{m} K_{ik}\delta_k} \tag{S3.4}$$

with $\sum_{j=1}^{m} R_{ij} = 1$. Using the relation and $\sum_{j=1}^{m} \delta_j = 1$ and $\sum_{i=1}^{n} \pi_j = 1$, it gives $\lambda = 1$. This leads to the stationary distribution $\delta$ at the coarse scale

$$\delta_j = \sum_{i=1}^{n} \pi_i R_{ij}. \tag{S3.5}$$

$R = \{R_{ij}\}$ maps $\pi$ to $\delta$, acting as a reduction operator. Following Bayes theorem,

$$K_{ij} = \frac{R_{ij}\pi_i}{\delta_j}. \tag{S3.6}$$

The operations $K$ and $R$ and stationary distribution $\delta$ can be computed using the EM-type procedure: (i) select an initial estimate for $K$ and $\delta$; (ii) E-step: compute ownership map $R$ using $R_{ij} = \frac{K_{ij}\delta_j}{\sum_{k=1}^{m} K_{ik}\delta_k}$; (iii) M-step: compute $K$ and $\delta$ using $\delta_j = \sum_{i=1}^{n} \pi_i R_{ij}$ and $K_{ij} = \frac{R_{ij}\pi_i}{\delta_j}$; repeat E- and M-steps until convergence.

The Markov transition matrix in the coarse-grained representation $\widetilde{M}$ follows

$$\widetilde{M} = \mathrm{diag}(\delta) K^{\intercal} \,\mathrm{diag}(K\delta)^{-1} K. \tag{S3.7}$$

We can generate a symmetric affinity matrix $\widetilde{A}$ that describes the interactions in the low-resolution network

$$\widetilde{A} = \widetilde{M}\,\mathrm{diag}(\delta). \tag{S3.8}$$

## S4 QROM based on direct quantization of classical ROM

There exist several polylog($N$)-depth implementations of QROM [40] with the cost of $O(N)$ qubits involved. Here, we introduce a direct quantization of the classical ROM which features polylog($N$) depth, and supports arbitrary trade-offs between circuit depth and qubit number.

### S4.1 1-of-$N$ decoder

A classical ROM contains 2 parts. Part 1 is a binary decoder, or more precisely a 1-of-$N$ decoder, which translates the binary address to a 1-of-$N$ representation. For instance, if the input address is $5 = |101\rangle$, then the output should be $|0000100...\rangle$ where only the 5th qubit has value 1. Quantum binary decoder can be implemented by a polylog($N$)-depth circuit with $O(N)$ qubits. The gate implementation is shown below where we start by considering a 1-of-2 decoder.

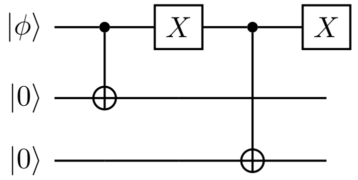


Figure 1: The 1-of-2 decoer.

Any 1-to-$2^n$ decoder can be constructed by applying 1-of-($2^{n-1}$) twice. For example, the 1-of-4 decoder can be made by 2 1-of-2 decoders.

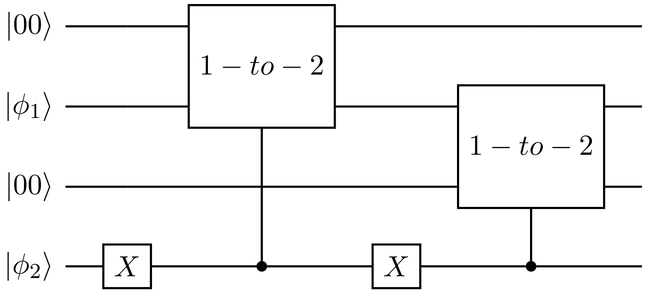


Figure 2: The 2-to-4 decoder.

### S4.2 Hard-coded data loader

Once the binary number is decoded as the 1-of-$N$ representation, the data can be loaded by $m$ layers of large OR-type CNOT gates which performs the $X$ gate if *any* of the control qubits is 1, where $m$ is the length of the data of each element. In this paper, $m$ represents the precision of initial positions of the atoms or residues.

The large OR-type CNOT gate can be implemented by $O(\log N)$ layers of OR gates and a single CNOT gate, thus is also depth-efficient.

### S4.3 State-based data loader

A more flexible method is to store the classical data in some data states that can be called, instead of hard-coding them as the gates, and apply CCNOT gates to copy them into the output qubits, as shown in Figure 4. Note that the CCNOT gates here are the normal CCNOT: if both control

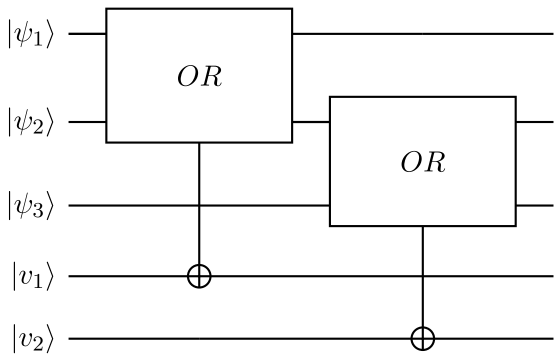


Figure 3: The data loader for the following dictionary: $\{1 \to 10, 2 \to 11, 3 \to 01\}$

qubits are in $|1\rangle$, then the $X$ gate is applied to the target qubit, unlike in the hard-coded data loader.

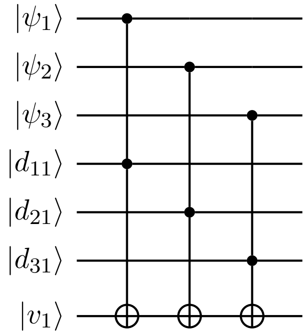


Figure 4: The state-based data loader for a dictionary of 3 indices with single-qubit data.

Similar techniques can be used to reduce its depth to $O(\log N \log M)$. $N$ CCNOT gates acting on the same target qubit can be considered as a large OR-CCNOT gate (the Pauli operator $X_j$ on the $j$th output qubit is applied if any pair of $|\psi_i\rangle$ and $|d_{ij}\rangle$) is in $|1\rangle|1\rangle$, which an be implemented by one layer of parallel AND gates and $O(\log N)$ layers of OR gates.

The construction described above has *polylogN*-depth and $O(N)$-width. However, on a specific platform implementing the algorithm, a narrower but deeper circuit might be preferred to increase its performance. Our QROM implementation based on hard-coded loader features a trade-off between qubit number and circuit depth, as shown in the following theorem.

**Theorem S4.1** (Width-depth trade-off of QROM)**.** *For arbitrary $k \in \{0, 1, \ldots, n\}$, there is a hard-coded QROM implementation with $O(2^{n-k})$ qubits and $O(2^k m \cdot poly(n))$ circuit depth, where $2^n$ is the number of indices, and $m$ is the number of bits of each data $v_i$ corresponding to the ith index.*

*Proof.* For $k = 0$, this is the original hard-coded version QROM, where $n$ bits of the input index is translated to the 1-of-$2^n$ format using a $poly(n)$-depth decoder and the data is loaded using $O(m)$ layers of $poly(n)$-depth OR-type CNOT gates. The total number of qubits is $O(2^n)$.

To reduce the qubit number by half, one can choose not to decode the most significant bit (MSB) in the 1-of-$N$ decoder, and run 2 different data loader circuits conditioned on different values of the MSB to load the information corresponding to MSB=0 and MSB=1, respectively, as shown in Figure 5. Such a reduction can be run for arbitrarily many significant bits, and for every bit the qubit number is halved while the circuit depth is doubled. Therefore, for any $k \in \{0, 1, \ldots, n\}$ the qubit number can be reduced to $O(2^{n-k})$, and the circuit depth becomes $O(2^k m \cdot poly(n))$ for $k$ times of trade-off. □

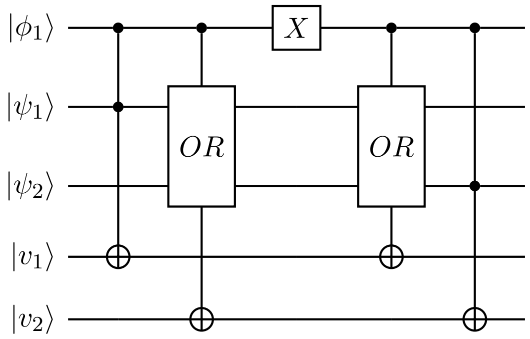


Figure 5: The data loader with a $k = 1$ depth-width trade-off for the following dictionary: $\{1 \to 10, 2 \to 11, 3 \to 11, 4 \to 01\}$

# S5 Initial state preparation theorems

## S5.1 The joint state preparation lemma

**Lemma S5.1** (Joint state preparation from Lemma 10 in Ref. [8])**.** *Assume we have access to the oracle $\mathcal{S}$ for d-sparse kernel matrix $H$ and diagonal mass matrix $M$, and the unitary $U_I$ that performs the map*

$$U_I |0\rangle |0\rangle = |0\rangle |\dot{\boldsymbol{u}}(0)\rangle , \qquad U_I |1\rangle |0\rangle = |1\rangle |\boldsymbol{u}(0)\rangle , \tag{S5.1}$$

*where*

$$|\boldsymbol{u}(0)\rangle \propto \sum_{j=1}^{N} \boldsymbol{u}_j(0) |j\rangle , \qquad |\dot{\boldsymbol{u}}(0)\rangle \propto \sum_{j=1}^{N} \dot{\boldsymbol{u}}_j(0) |j\rangle , \tag{S5.2}$$

*are normalized states. There exists a quantum algorithm that prepares the state*

$$|\psi(0))\rangle := \frac{1}{\sqrt{2E}}[\dot{\boldsymbol{y}}(0), i\sqrt{A}\boldsymbol{y}(0)]^T, \tag{S5.3}$$

*where $\boldsymbol{y}(0) = \sqrt{M}\boldsymbol{u}(0)$ and $A := (\sqrt{M})^{-1}K(\sqrt{M})^{-1}$, and $E$ is the total energy. The quantum circuit makes $Q_{\text{ini}} = \mathcal{O}(\frac{E_{\max}d}{E})$ uses of $\mathcal{S}$, $U_I$, and its inverses, in addition to*

$$G_{\text{ini}} = \mathcal{O}\Big(\frac{E_{\max}d}{E}\,\text{polylog}(\frac{NE_{\max}d}{E\epsilon})\Big) \tag{S5.4}$$

*two-qubit gates. Here $E_{\max} := \frac{m_{\max}}{2}\sum_j(\dot{\boldsymbol{u}}_j(0))^2 + \frac{\kappa_{\max}}{2}\sum_j(\boldsymbol{u}_j(0))^2$.*

### S5.2 Proof of Theorem 1

To prove Theorem 1, our first finding is the following lemma.

**Lemma S5.2** (Distribution of Gaussian random amplitude states)**.** *Gaussian random amplitude states corresponding to any uncertainty $\mu > 0$ follow the same uniform distribution of real-amplitude states.*

*Proof.* We notice that one sample of *unnormalized* Gaussian random amplitude state of $n$ qubits with uncertainty $\mu$ can be represented by an array of $2^n$ real numbers, denoted by $\boldsymbol{\alpha} = (\alpha_0, \ldots, \alpha_{2^n-1})^{\mathrm{T}}$, with $\alpha_i \sim \mathcal{N}(0, \mu)$ for all $i$. The unnormalized state corresponding to $\boldsymbol{\alpha}$ is

$$|\psi_{\boldsymbol{\alpha}}\rangle = \sum_{i=0}^{2^n-1} \alpha_i |i\rangle . \tag{S5.5}$$

The probability density corresponding to $|\psi_{\boldsymbol{\alpha}}\rangle$ is

$$f(|\psi_{\boldsymbol{\alpha}}\rangle) = \prod_{i=0}^{2^n-1} \frac{1}{\sqrt{2\pi\mu^2}} \exp\left(-\frac{\alpha_i^2}{2\mu^2}\right) = \left(2\pi\mu^2\right)^{-2^{n-1}} \exp\left(-\frac{1}{2\mu^2}\sum_{i=0}^{2^{n-1}} \alpha_i^2\right). \tag{S5.6}$$

The normalized version of $|\psi_{\boldsymbol{\alpha}}\rangle$ is simply $\left|\tilde{\psi}_{\boldsymbol{\alpha}}\right\rangle := \frac{1}{\sqrt{\sum_{i=0}^{2^n-1}\alpha_i^2}} |\psi_{\boldsymbol{\alpha}}\rangle$. We then observe that the probability density corresponding to $\left|\tilde{\psi}_{\boldsymbol{\alpha}}\right\rangle$ is a value depending only on $\mu$:

$$f\left(\left|\tilde{\psi}_{\boldsymbol{\alpha}}\right\rangle\right) = \left(2\pi\mu^2\right)^{-2^{n-1}} \exp\left(-\frac{1}{2\mu^2}\sum_{i=0}^{2^{n-1}} \frac{\alpha_i^2}{\sum_{j=0}^{2^{n-1}} \alpha_j^2}\right) = \left(2\pi\mu^2\right)^{-2^{n-1}} e^{-\frac{1}{2\mu^2}}. \tag{S5.7}$$

Therefore, any unnormalized version of $|\psi_{\boldsymbol{\alpha}}\rangle$ can be written as $\gamma\left|\tilde{\psi}_{\boldsymbol{\alpha}}\right\rangle$ with $\gamma \neq 0$ and has probability density

$$f\left(\gamma\left|\tilde{\psi}_{\boldsymbol{\alpha}}\right\rangle\right) = \left(2\pi\mu^2\right)^{-2^{n-1}} e^{-\frac{\gamma^2}{2\mu^2}}. \tag{S5.8}$$

The probability density of all states equivalent to $|\psi_{\boldsymbol{\alpha}}\rangle$ can also be calculated by integrating over $\gamma \in (-\infty, 0) \cup (0, \infty)$ since $\gamma = 0$ is forbidden:

$$\Pr(|\psi_{\boldsymbol{\alpha}}\rangle) = \int_{\gamma=-\infty}^{\infty} f\left(\gamma\left|\tilde{\psi}_{\boldsymbol{\alpha}}\right\rangle\right)(1-\delta(\gamma))d\gamma = \int_{\gamma=-\infty}^{\infty} \left(2\pi\mu^2\right)^{-2^{n-1}} (1-\delta(\gamma)) e^{-\frac{\gamma^2}{2\mu^2}} d\gamma \tag{S5.9}$$

which is again a value independent of $\boldsymbol{\alpha}$. This implies that the probability of obtaining any $\left|\tilde{\psi}_{\boldsymbol{\alpha}}\right\rangle$ from the distribution of Gaussian random amplitude states is the same. Therefore, the distribution of Gaussian random amplitude states is simply the uniform distribution of all real-amplitude normalized states. □

Letting $p := \Pr(|\psi_{\boldsymbol{\alpha}}\rangle)$ and using the fact that $|\psi_{\boldsymbol{\alpha}}\rangle$ is normalized when $\sum_{i=0}^{2^n-1} \alpha_i^2 = 1$, we can write down the density matrix describing the distribution of initial states and decompose it in the

computational basis:

$$\begin{aligned}\rho_{\mathrm{G}} &= \int_{\sum_{i=0}^{2^n-1} \alpha_i^2=1} \Pr(|\psi_{\boldsymbol{\alpha}}\rangle) \, |\psi_{\boldsymbol{\alpha}}\rangle \langle \psi_{\boldsymbol{\alpha}}| \, d\boldsymbol{\alpha} \\ &= p \left[ \sum_{j=0}^{2^n-1} \int_{\sum_{i=0}^{2^n-1} \alpha_i^2=1} \alpha_j^2 \, |j\rangle \langle j| \, d\boldsymbol{\alpha} + \sum_{j,k=0}^{2^n-1} \int_{\sum_{i=0}^{2^n-1} \alpha_i^2=1} \alpha_j \alpha_k \, |j\rangle \langle k| \, d\boldsymbol{\alpha} \right] \\ &= \frac{1}{2^n} \sum_{j=0}^{2^n-1} |j\rangle \langle j| \end{aligned} \tag{S5.10}$$

where all non-diagonal terms have 0 amplitude in the density matrix since $\alpha_j \alpha_k$ is an odd function when integrating over any of them, and all diagonal terms have equal weight since $\int_{\sum_{i=0}^{2^n-1} \alpha_i^2=1} \alpha_j^2$ is the same for all $j$.

Therefore, if we wish to compute any average quantity over all possible initial states, it suffices to prepare the maximally mixed state by preparing

$$|\psi_{\mathrm{pure}}\rangle = \frac{1}{\sqrt{2^n}} \sum_{j=0}^{2^n-1} |j\rangle \, |j\rangle \tag{S5.11}$$

and discarding the second register. $|\psi_{\mathrm{pure}}\rangle$ can be easily prepared by performing Hadamard gates on all qubits and applying CNOT gates between qubits in register 1 and register 2. This concludes our proof of Theorem 1.

### S5.3 Quantum mean estimation

We notice that a $|\psi_{\mathrm{pure}}\rangle$ is the purification of $\rho_{\mathrm{G}}$, which can also be used to estimate average quantities over the ensemble, as shown below. Let $U$ be the quantum simulation algorithm and $O$ be the observable to be measured. The expectation value of $O$ over the whole ensemble of Gaussian random amplitude states is

$$\mathrm{Tr}\Big[U \rho_{\mathrm{G}} U^\dagger O\Big] = \frac{1}{2^n} \sum_{j=0}^{2^n-1} \langle j | U^\dagger O U | j \rangle. \tag{S5.12}$$

Now, if we run $I \otimes U$ on $|\psi_{\mathrm{pure}}\rangle$ and measure $I \otimes O$, we obtain

$$\mathrm{Tr}\Big[I \otimes U \cdot |\psi_{\mathrm{pure}}\rangle \langle \psi_{\mathrm{pure}}| \cdot I \otimes U^\dagger \cdot I \otimes O\Big] = \frac{1}{2^n} \sum_{j=0}^{2^n-1} \langle j|j\rangle \langle j | U^\dagger O U | j \rangle = \mathrm{Tr}\Big[U \rho_{\mathrm{G}} U^\dagger O\Big], \tag{S5.13}$$

which is the same mean value. Note that we have access to both the circuit preparing $U|\psi_{\mathrm{pure}}\rangle$ and its reverse. This implies that we can employ *quantum mean estimation* [14, 18, 33] to achieve a quadratic improvement in the sample complexity of estimating any average value over the whole distribution.

### S5.4 Proof of Lemma 2

We first write $p_l(\theta_i)$ as

$$p_l(\theta_i) = \frac{1}{\zeta_l} \sin^{2^{l'}-1}(2\theta_i) \tag{S5.14}$$

where the normalization factor $\zeta_l$ can be computed by integrating $\sin^{2^{l'}-1}(x)$:

$$\zeta_l = \int_0^{\pi/2} \sin^{2^{l'}-1}(2x)dx = \frac{1}{2}\int_0^{\pi} \sin^{2^{l'}-1}(x)dx = 2^{2^{l'}-l'-1}\left[\binom{2^{l'}}{2^{l'-1}}\right]^{-1}. \tag{S5.15}$$

Recall that we focus on the case of $l' \gg \log n$. Using

$$\frac{2^{2^{l'}}}{\sqrt{\pi\left(2^{l'-1}+\frac{1}{3}\right)}} \le \binom{2^{l'}}{2^{l'-1}} \le \frac{2^{2^{l'}}}{\sqrt{\pi\left(2^{l'-1}+\frac{1}{4}\right)}}, \tag{S5.16}$$

we can rewrite $\zeta_l$ as

$$\zeta_l = \sqrt{\pi}\cdot 2^{-l'-1}\cdot\left(2^{\frac{l'-1}{2}} + \mathcal{O}\left(2^{\frac{-l'+1}{2}}\right)\right) = 2^{\frac{-l'-3}{2}}\sqrt{\pi} + \mathcal{O}\left(2^{\frac{-3l'}{2}}\right). \tag{S5.17}$$

We use a step function (piecewise constant function) to construct $Q_l \cdot q_l(x)$. Since $p_l(x)$ is peaked at $x = \pi/4$, we let $Q_l \cdot q_l(x) = p_l(\pi/4) = \zeta_l^{-1}$ in a small region around $x = \pi/4$. We choose the region to be $[\pi/4 - \zeta_l, \pi/4 + \zeta_l]$. One can now see that

$$\int_{\pi/4-\zeta_l}^{\pi/4+\zeta_l} Q_l \cdot q_l(x)dx = 2, \tag{S5.18}$$

while

$$\begin{aligned}
\int_{\pi/4-\zeta_l}^{\pi/4+\zeta_l} p_l(x)dx &\ge 2\zeta_l \cdot p_l(\pi/4-\zeta_l) \\
&= 2\sin^{2^{l'}-1}(\pi/2 - 2\zeta_l) \\
&= 2\left[1 - 2\zeta_l^2 + \frac{2}{3}\zeta_l^4 - \dots\right]^{2^{l'-1}} \\
&= 2\left[1 - \frac{\pi}{4}2^{-l'} + \mathcal{O}\left(2^{-2l'}\right)\right]^{2^{l'-1}} \\
&\ge 2\left[1 - \frac{\pi}{4}2^{-l'}\right]^{2^{l'}-1} \\
&= 2e^{-\pi/4} + \mathcal{O}\left(2^{-l'}\right) \approx 0.91 + \mathcal{O}\left(2^{-l'}\right)
\end{aligned} \tag{S5.19}$$

which is a constant close to 1 when $l'$ is large. In this range, our $Q_l \cdot q_l(x)$ performs well, since the ratio between the integral of the real distribution and the proposal distribution is at least 0.45 when $l'$ is large.

Next, we construct $Q \cdot q_l(x)$ in the region to the left side of $\pi/4 - \zeta_l$ and to the right side of $\pi/4 + \zeta_l$. We consider the range $x \in [\pi/4 - 2\zeta_l, \pi/4 - \zeta_l] \cup [\pi/4 + \zeta_l, \pi/4 + 2\zeta_l]$ and simply let $Q_l \cdot q_l(x) = p_l(\pi/4 - \zeta_l)$ for $x$ in this range. Similarly, the $k$th region to consider is $x \in$

$[\pi/4-k\zeta_l, \pi/4-(k-1)\zeta_l]\cup[\pi/4+(k-1)\zeta_l, \pi/4+k\zeta_l]$, and the value of $Q_l\cdot q_l(x)$ is $p_l(\pi/4-(k-1)\zeta_l)$. We proceed to increase $k$ one by one, until we reach $k=k_T$ satisfying $p_l(\pi/4-k_T\zeta_l)=\mathcal{O}\left(2^{-l'}\right)$. Since that the probability of obtaining $x\in[0,\pi/4-k_T\zeta_l]$ is exponentially small, we can simply let $Q_lq_l(x)=p_l(\pi/4-k_T\zeta_l)$ for $x\in[0,\pi/4-k_T\zeta_l]\cup[\pi/4+k_T\zeta_l,\pi/2]$. We can compute $k_T$ by

$$p_l(\pi/4-k_T\zeta_l)=\frac{1}{\zeta_l}\left[1-\frac{k^2\pi}{4}2^{-l'}\right]^{2^{l'}-1}=\mathcal{O}\left(2^{\frac{l'}{2}}e^{-\frac{k^2\pi}{4}}\right)\le\mathcal{O}\left(2^{-l'}\right) \tag{S5.20}$$

which implies that $k_T=\mathcal{O}(\sqrt{l})=\mathcal{O}(\sqrt{n})$. Therefore, $Q_lq_l(x)$ is efficiently computable, integrable, and its integration is efficiently invertible, since $Q_lq_l(x)$ is a step function of at most $\mathcal{O}(\sqrt{n})$ steps.

Finally, we compute the success probability of rejection sampling, $p_{\mathrm{suc},l}$, which is related to the area enclosed by $Q_lp_l(x)$. We first compute an upper bound of the area enclosed by it in the $k$th range, i.e., $[\pi/4-k\zeta_l,\pi/4-(k-1)\zeta_l]\cup[\pi/4+(k-1)\zeta_l,\pi/4+k\zeta_l]$:

$$\begin{aligned}2\int_{\pi/4-k\zeta_l}^{\pi/4-(k-1)\zeta_l}Q\cdot q_l(x)dx&=2\zeta_lq_l(\pi/4-(k-1)\zeta_l)\\&=2\left[1-\frac{(k-1)^2\pi}{4}2^{-l'}+\mathcal{O}\left(2^{-2l'}\right)\right]^{2^{l'}-1}\\&\le2\left[1-\frac{(k-1)^2\pi}{2}2^{-l'}+\mathcal{O}\left(2^{-2l'}\right)\right]^{2^{l'}-1}\\&=e^{-\frac{(k-1)^2\pi}{2}}+\mathcal{O}\left(2^{-l'}\right).\end{aligned} \tag{S5.21}$$

Therefore, the total area can be upper bounded by

$$\int_0^{\pi/2}Q_lp_l(x)dx\le2\sum_{k=1}^{\mathcal{O}(\sqrt{n})}e^{-\frac{(k-1)^2\pi}{2}}=\mathcal{O}(1), \tag{S5.22}$$

a constant. This implies that the rejection sampling success probability satisfies

$$p_{\mathrm{suc},l}=\frac{\int_0^{\pi/2}p_l(x)dx}{\int_0^{\pi/2}Q_lp_l(x)dx}\ge\mathcal{O}(1). \tag{S5.23}$$

## S5.5 Completing the quantized rejection sampling procedure

Using the pseudo-random number $r(s,i)$, we can invert the cdf of $q_l(x)$ to obtain $s_q(i)$ which is a sample from $q_l(x)$:

$$\sum_{i\in\{0,1\}^{l-1}}\alpha_{l,i}\left|i\right\rangle\left|r(s,i)\right\rangle\left|00\ldots0\right\rangle\mapsto\sum_{i\in\{0,1\}^{l-1}}\alpha_{l,i}\left|i\right\rangle\left|r(s,i)\right\rangle\left|s_q(i)\right\rangle\ \mapsto\sum_{i\in\{0,1\}^{l-1}}\alpha_{l,i}\left|i\right\rangle\left|00\ldots0\right\rangle\left|s_q(i)\right\rangle \tag{S5.24}$$

where in the last step we apply the inverse circuit of the quantized CBRNG. Next, we determine whether $s_q(i)$ should be accepted or rejected. We uniformly sample $r_q(s',i)$ from $[0,Q_lq_l(s_q(i))]$

using another CBRNG with seed $s'$:

$$\sum_{i\in\{0,1\}^{l-1}} \alpha_{l,i} |i\rangle |s_q(i)\rangle |00\ldots0\rangle |00\ldots0\rangle \mapsto \sum_{i\in\{0,1\}^{l-1}} \alpha_{l,i} |i\rangle |s_q(i)\rangle \left|r_q(s',i)\right\rangle |0\rangle$$
$$\mapsto \sum_{i\in\{0,1\}^{l-1}} \alpha_{l,i} |i\rangle |s_q(i)\rangle \left|r_q(s',i)\right\rangle \left|r_q(s',i) \le p_l(s_q(i))\right\rangle \tag{S5.25}$$

Now, if $r_q(s',i) \le p_l(s_q(i))$, then $s_q(i)$ is accepted as $\theta_i$. Otherwise, we need to repeat the above process using another set of random numbers, $r(s, i + j \cdot 2^n)$ and $r_q(s', i + j \cdot 2^n)$ where $j = 1$ for the second round, and $j = k - 1$ for the $k$th round if necessary. For each round, we also need to use new ancilla registers to store $r$,$s_q$, and $r_q$ values. Fortunately, this rejection sampling process only needs to be repeated $\mathcal{O}(n)$ times for the $l$th qubit to accept all $\theta_i$s with high probability.

**Lemma S5.3.** *If we need all $\theta_i$ to be accepted with a constant high probability after $N_l$ rounds, it suffices to have $N_l = \mathcal{O}(n)$, a constant value independent of $l$.*

*Proof.* Since the probability for each sample to be accepted is $p_{\text{suc},l} = \mathcal{O}(1)$, the probability of being accepted after $N_l$ rounds is $1 - (1 - p_{\text{suc},l})^{N_l}$. Therefore, if $N_l = 2vn$ with $v > 1$ being a constant satisfying $(1 - p_{\text{suc},l})^v < 1/2$, we can achieve $(1 - p_{\text{suc},l})^{N_l} = \left((1 - p_{\text{suc},l})^{2v}\right)^n \ll 2^{-2n}$. Now, one can use binomial approximation to show that the probability for all $2^{l-1}$ values to be accepted is

$$\left(1 - (1 - p_{\text{suc},l})^{N_l}\right)^{2^{l-1}} \approx 1 - 2^{l-1}(1 - p_{\text{suc},l})^{N_l} \ge 1 - 2^{l-1-2n} \ge 1 - \mathcal{O}(2^{-n}), \tag{S5.26}$$

which is arbitrarily close to 1. Therefore, it suffices to apply $\mathcal{O}(n)$ rounds of the above rejection sampling procedure for each binary data loader to generate all $\theta_i$s in superposition. □

$\mathcal{O}(n)$ repetitions require $\mathcal{O}(n^2)$ random seeds in total, and the total number of rounds (or the circuit depth) is $\mathcal{O}(n^2)$. Since all random seeds are determined classically and loaded into the quantum circuit, all random numbers and $r_q(s, i + j \cdot 2^n)$ values are generated deterministically, and all scratch qubits can be erased, which allows us to obtain $\sum_{i\in\{0,1\}^{l-1}} \alpha_{l,i} |i\rangle |\theta_i\rangle$. Finally, we can use binary data loader to complete the rotation and uncompute the $\theta_i$ from $i$ by inverting the sampling circuit:

$$\sum_{i\in\{0,1\}^{l-1}} \alpha_{l,i} |i\rangle |\theta_i\rangle \mapsto \sum_{i\in\{0,1\}^{l-1}} \alpha_{l,i} \left(\cos(\theta_i) |i0\rangle + \sin(\theta_i) |i1\rangle\right) |\theta_i\rangle$$
$$\mapsto \sum_{i\in\{0,1\}^{l-1}} \alpha_{l,i} \left(\cos(\theta_i) |i0\rangle + \sin(\theta_i) |i1\rangle\right) |0\rangle . \tag{S5.27}$$

Since we only need one ancilla register to store $\theta_i$s and it can be reused by the next data loader, we only need poly$(n)$ ancilla qubits to store the seed, instead of $\mathcal{O}(2^n)$ qubits for the whole $\boldsymbol{\theta}$ vector. The gate complexity of the whole process is also poly$(n)$.

# S6 Matrix loading with efficient modification

In this section, we discuss the construction of data access oracle supporting efficient molecule-structure modification.

We store each row of the Hamiltonian $H$ using a binary tree, which allows for efficient quantum readout and classical modification of every row. This data structure is used in Ref. [59] to simulate the dynamics of dense Hamiltonians. Note that here we directly work on the Hamiltonian $H$ as defined in Ref. [8] which contains information on both spring constants and masses of all elements.

Let $T^i$ represent a binary tree storing the $i$th row of $H$, thus $T := (T^1, T^2, \ldots, T^N)$ stores the whole $H$ matrix. Nodes of $T^i$ are real or complex values, and they are indexed by a binary string $s \in \{0,1\}^1 \cup \{0,1\}^2 \cup \cdots \cup \{0,1\}^n$ (recall that $n = \log N$). The structure of $T^i$ is defined as follows, where $|\cdot|$ denotes the number of bits in the binary string.

- If $|s| = n$, then $s$ corresponds to a leaf node. Its value satisfies $T^i_s = H^*_{i,s}$.
- If $|s| < n$, then $s$ corresponds to a branch node, and its left-child node and right-child node are $s0$ and $s1$ respectively. Its value is real and satisfies $T^i_s = |T^i_{s0}| + |T^i_{s1}|$.

In other words, each branch node of $T^i$ represents the sum of $|H_{i,j}|$ for a specific range of $j$. If we construct the QROM access to elements of every $T^i$ binary tree, then we can employ the algorithm of Refs. [40, 59] to produce a quantum state that is proportional to the $i$th row of the matrix with high probability:

$$|i\rangle |0\rangle^{\otimes n} \to |i\rangle \sum_{j=0}^{N-1} \sqrt{H^*_{i,j}}\, |j\rangle \tag{S6.1}$$

using a $\mathcal{O}(n^2)$ depth quantum circuit.

Recall in Ref. [8], $H$ is defined as

$$H = -\begin{pmatrix} 0 & B \\ B^\dagger & 0 \end{pmatrix} \tag{S6.2}$$

and $B$ satisfies

$$\begin{aligned} \sqrt{M} B\, |j, j\rangle &= \sqrt{\kappa_{jj}}\, |j\rangle \\ \sqrt{M} B\, |j, k\rangle &= \sqrt{\kappa_{jk}}(|j\rangle - |k\rangle) \end{aligned} \tag{S6.3}$$

Therefore, the matrix $B$ stores a similar amount of information as the $K$ matrix, except that the inverse mass of each spring is multiplied by the spring coefficients.

We claim that the binary-tree data structure for $H$ above supports the following efficient modifications of the protein structure. Here focus on *engineering complexity*, which is defined as the number of values stored in QROM to be modified, since constructing a hard-coded QROM is an expensive engineering effort. Note that according to Refs. [40, 59], modification of each matrix element has polylog($N$) engineering complexity. Hence we only consider the number of matrix elements to be modified in the following discussions.

1. Mass modification. If the mass of a single element of the system needs to be modified, then a total number of $\mathcal{O}(d)$ matrix elements need to be modified.
2. Position modification. If the position of one element is changed, then all spring constants connecting to it need to be changed, which is also $\mathcal{O}(d)$.

3. Add an element. First, there needs to be a new row of $B$, thus a new binary tree $T^{N+1}$ to store the row. $T^{N+1}$ has $\mathcal{O}(d)$ non-zero leaf nodes, thus the number of leaf node modifications is $\mathcal{O}(d)$. Second, every row that has connection to the new node should have a new leaf node, which is also $\mathcal{O}(d)$. The total number of modifications is $\mathcal{O}(d)$.

4. Remove an element. First, the tree $T^i$ needs to be deleted, where $i$ is the index of the element. For every other tree that has a connection with the $i$th element, one leaf node needs to be removed, which leads to an overall number of leaf node modifications $\mathcal{O}(d)$. Note that in such a process, what we are essentially doing is to remove all springs connecting the $i$th element and the others. Therefore, when preparing the initial state, one can still assign position and velocity for the element, and both values will not change during the process of simulation, thus making no contribution to the dynamics of the system.

## S7 Simulating protein dynamics on quantum computers

In this section, we consider quantum algorithms for simulating protein dynamics with non-Hermitian structures and external forces or noises. For the standard harmonic approximation model, we perform Hamiltonian simulation to propagate initial state $|\psi(0)\rangle\rangle$ to a target final state $|\psi(T)\rangle\rangle$, which includes information on the motions of proteins. For general non-Hermitian dynamics, we consider quantum linear ODE solvers or Linear Combination of Hamiltonian Simulations (LCHS) to produce the final states or the Feymann-Kac history states (known as the dense output [50]). For Langevin dynamics, we apply open quantum system simulations to produce the final states described by the density matrix.

As introduced in Section **??**, we are interested in the harmonic approximation model near by an equilibrium as in (S2.1)

$$m_i \ddot{u}_i = -\sum_{j=1}^{N} K_{ij} u_j, \tag{S7.1}$$

and the harmonic approximation model away from an equilibrium as in (S2.19)

$$m_i \ddot{u}_i = -\sum_{j=1}^{N} K_{ij} u_j + F_i. \tag{S7.2}$$

We can apply the Hamiltonian simulation algorithm to produce the final state of the former model. We need to apply quantum linear ODE solvers to simulate the later model, or to produce the history state of the former model.

### S7.1 Hamiltonian Simulation

Our goal is to develop a quantum algorithm to efficiently simulate protein dynamics. In our problem formulation, the input and output are quantum states whose amplitudes encode the velocities and displacements of the protein molecules. Inspired by [8], we consider the Hamiltonian simulation

algorithm for protein dynamics, modeled by the equation of motions. We reproduce the harmonic oscillator system in (S2.1) as

$$M\frac{\mathrm{d}^2\boldsymbol{u}(t)}{\mathrm{d}t^2} + K\boldsymbol{u}(t) = 0. \tag{S7.3}$$

We consider a change of variables

$$\boldsymbol{y}(t) = \sqrt{M}\boldsymbol{u}(t), \tag{S7.4}$$

where $\sqrt{M}$ is a matrix square root, which is a trivial operation since $M$ is diagonal. This allows us to eliminate $M$ from the equation and rewrite the dynamics as

$$\ddot{\boldsymbol{y}}(t) + A\boldsymbol{y}(t) = 0, \tag{S7.5}$$

where $A \coloneqq (\sqrt{M})^{-1}K(\sqrt{M})^{-1}$. The key observation is that any solution $\boldsymbol{y}(t)$ of (S7.5) should also satisfy

$$\ddot{\boldsymbol{y}}(t) + i\sqrt{A}\dot{\boldsymbol{y}}(t) = i\sqrt{A}\Big(\dot{\boldsymbol{y}}(t) + \sqrt{A}\boldsymbol{y}(t)\Big), \tag{S7.6}$$

hence its solution is given by

$$\dot{\boldsymbol{y}}(t) + \sqrt{A}\boldsymbol{y}(t) = e^{i\sqrt{A}t}\Big(\dot{\boldsymbol{y}}(0) + \sqrt{A}\boldsymbol{y}(0)\Big). \tag{S7.7}$$

As a result, the solution at time $t$ can be obtained by simulating $e^{i\sqrt{A}t}$ via a Hamiltonian simulation algorithm. More specifically, suppose that we have access to $A$ rather than $\sqrt{A}$. Following the incidence matrix approach [19, 8], we aim to construct a matrix $B$ such that $BB^\dagger = A$ and a block Hamiltonian

$$H = -\begin{bmatrix} 0 & B \\ B^\dagger & 0 \end{bmatrix}. \tag{S7.8}$$

We notice that the first block of $H^2$ is $A$. We turn to simulate the Schrödinger equation

$$\mathrm{i}\frac{\mathrm{d}}{\mathrm{d}t}\left|\psi(t)\right\rangle = H\left|\psi(t)\right\rangle. \tag{S7.9}$$

with

$$|\psi(t)\rangle \coloneqq \frac{1}{\sqrt{2E}}[\dot{\boldsymbol{y}}(t), iB^\dagger\boldsymbol{y}(t)]^T. \tag{S7.10}$$

On natural choice of $B$ is $-\sqrt{A}$. But the choice is clearly not unique. In particular, one can pick a rectangular matrix to fulfill the condition $BB^\dagger = A$. We follow the choice in [8], where

$$\sqrt{M}B|j,k\rangle = \begin{cases} \sqrt{K_{jk}}(|j\rangle - |k\rangle), & j < k \\ \sqrt{K_{jj}}|j\rangle, & i = j. \end{cases} \tag{S7.11}$$

This choice satisfies $\sqrt{M}B(\sqrt{M}B)^\dagger = K$ and hence $BB^\dagger = A$. So we can block encode $\sqrt{M}B$ and then divide it by $\sqrt{M}^{-1}$ to obtain $B$.

**Problem 1.** *We consider the harmonic oscillator system (S7.3) and reshape it as (S7.5). Let $M$ be an $N \times N$ diagonal matrix with positive diagonal elements, and $K$ be an $N \times N$ real symmetric, positive-defnite, and d-sparse matrix. Define the normalized state*

$$|\psi(t))\rangle := \frac{1}{\sqrt{2E}}[\dot{\boldsymbol{y}}(t), iB^{\dagger}\boldsymbol{y}(t)]^T, \tag{S7.12}$$

*where $E > 0$ is a normalizing constant. Assume we have unitaries $U_M$ and $U_F$ that prepare $M$ and $K$, and a unitary $U_I$ that prepares the initial state $|\psi(0))\rangle$. Given $T > 0$, the goal is to produce $|\psi(T))\rangle$ within $\ell_2$ error tolerance $\epsilon$.*

Here we are interested in producing the state $|\psi(t))\rangle$ at a certain time $t$. This state encodes the velocities ($\dot{\boldsymbol{y}}(t)$) and displacements ($\boldsymbol{y}(t)$) of the protein molecules, hence it can be used to estimate the kinetic or potential energies.

The state-of-the-art Hamiltonian simulation algorithm can propagate $e^{iHt}$ with $\mathcal{O}(\|H\|t + \log(1/\epsilon))$ queries to the oracles of $H$ [51]. Based on the discussion above, especially Eqs. (S7.8) and (S7.11), a direct estimate is as follows: $\|H\| = \sqrt{\kappa_A}$, $\kappa_A = K_{\max}/m_{\min}$ with $m_{\max} \geqslant m_j \geqslant m_{\min} > 0$, and $K_{\max} \geqslant K_{jk}$. We reproduce the complexity of Hamiltonian simulation algorithm [8] as below.

**Theorem S7.1** (Theorem 1 of [8])**.** *Problem 1 can be solved with a quantum algorithm that makes*

$$\mathcal{O}\Big(\sqrt{\kappa_A}T + \log(1/\epsilon)\Big) \tag{S7.13}$$

*queries to the unitaries $U_M$ and $U_F$ that prepare $M$ and $F$, respectively, and one query to the unitary $U_I$ that prepares $\boldsymbol{x}(0)$, where $\kappa_A = K_{\max}/m_{\min}$, $m_{\max} \geqslant m_j \geqslant m_{\min} > 0$, and $K_{\max} \geqslant K_{jk}$. The one- or two-qubit gate complexity is larger by a poly-logarithmic factor.*

## S7.2 LCHS Method for steered protein dynamics

We now consider the normal mode dynamics under a mechanical force (S2.19). We reproduce it as

$$M\frac{\mathrm{d}^2\boldsymbol{u}(t)}{\mathrm{d}t^2} + K\boldsymbol{u}(t) = F. \tag{S7.14}$$

We consider a change of variables

$$\boldsymbol{y}(t) = \sqrt{M}\boldsymbol{u}(t), \tag{S7.15}$$

that allows us to rewrite the dynamics as

$$\ddot{\boldsymbol{y}}(t) + A\boldsymbol{y}(t) = \boldsymbol{b}, \tag{S7.16}$$

where $A := (\sqrt{M})^{-1}K(\sqrt{M})^{-1}$ and $\boldsymbol{b} := M^{-1}F$. Any solution $y(t)$ satisfies

$$\ddot{y}(t) + i\sqrt{A}\dot{y}(t) = i\sqrt{A}\Big(\dot{y}(t) + \sqrt{A}y(t)\Big) + \boldsymbol{b}, \tag{S7.17}$$

hence its solution is

$$\dot{y}(t) + \sqrt{A}y(t) = e^{i\sqrt{A}t}\Big(\dot{y}(0) + \sqrt{A}y(0)\Big) + \int_0^t e^{i\sqrt{A}t}b(t-s)\mathrm{d}s. \tag{S7.18}$$

This is a non-unitary dynamics and can be viewed as linear combination of Hamiltonian simulation.

Similarly, we cannot have access to $\sqrt{A}$, so we aim to construct a matrix $B$ such that $BB^\dagger = A$ and a block Hamiltonian

$$H = -\begin{bmatrix} 0 & B \\ B^\dagger & 0 \end{bmatrix}. \tag{S7.19}$$

We notice that the first block of $H^2$ is $A$. We turn to simulate the system of linear ODEs

$$\frac{\mathrm{d}}{\mathrm{d}t}|\psi(t))\rangle = -iH|\psi(t))\rangle + |\bar{b}\rangle. \tag{S7.20}$$

with

$$|\psi(t))\rangle := \frac{1}{\sqrt{2E}}[\dot{\boldsymbol{y}}(t), iB^\dagger \boldsymbol{y}(t)]^T. \tag{S7.21}$$

and

$$|\bar{b}\rangle := [\boldsymbol{b}(t), 0]^T. \tag{S7.22}$$

We describe the problem as follows.

**Problem 2.** *We consider the inhomogeneous harmonic oscillator system (S7.14). Under the same assumption of Problem 1, the goal is to produce $|\psi(T)\rangle$ within $\ell_2$ error tolerance $\epsilon$.*

Due to the inhomogeneous term in the differential equation, we cannot directly apply the standard Hamiltonian simulation in Theorem S7.1. Instead, we can apply the Theorem S7.3 to the final state problem or the history state problem.

We can also apply the Linear Combination of Hamiltonian Simulation (LCHS) to produce the final state with near-optimal dependence on all parameters [3, 2]. Compared to the Quantum Linear ODE Solver in Theorem S7.3, the LCHS method can significantly reduce the state preparation cost.

**Theorem S7.2** (Theorem 2 of [2])**.** *Problem 2 can be solved with a quantum algorithm that makes*

$$\mathcal{O}\left(q\sqrt{\kappa_A}T\log^{1+1/\beta}(\frac{1}{\epsilon})\right) \tag{S7.23}$$

*queries to the unitaries $U_M$ and $U_F$ that prepare $M$ and $F$, and $\mathcal{O}(q)$ queries to the unitaries $U_I$ and $U_b$ that prepare $\boldsymbol{x}(0)$ and $\boldsymbol{b}(t)$, where $\kappa_A = K_{\max}/m_{\min}$, $m_{\max} \geqslant m_j \geqslant m_{\min} > 0$, $K_{\max} \geqslant K_{jk}$, $q = \frac{\|\boldsymbol{x}_0\|+\|\boldsymbol{b}\|_{L^1}}{\|\boldsymbol{x}(T)\|}$, and $\|\boldsymbol{b}\|_{L^1} = \int_0^T \boldsymbol{b}(s)ds$, $\beta \in (0,1)$. The one- or two-qubit gate complexity is larger by a poly-logarithmic factor.*

In our case, we have Hermitian matrix $A(t) = H(t)$.

## S7.3 Quantum Linear ODE Solver for the dense outputs

We next consider the target of producing the history state of the protein dynamics. The general non-unitary process requires the usage of the quantum linear ODE solver. We again consider the general inhomogeneous ODE system (S7.14)

$$M\frac{\mathrm{d}^2\boldsymbol{u}(t)}{\mathrm{d}t^2} + K\boldsymbol{u}(t) = F. \tag{S7.24}$$

Given an initial condition $|\psi(t))\rangle$, we divide the time interval $[0,T]$ into $N_t = \mathcal{O}(T\log(1/\epsilon))$ sub-intervals, with $0 = t_0 < t_1 < \ldots < t_{N_t} = T$, $h_k = t_{k+1} - t_k$, where the nodes $\{t_k\}$ can be constructed by certain quadrature rules. For a time-independent Hamiltonian $H$, we construct $(N_t+1)n \times (N_t+1)n$ linear system

$$L|\Psi\rangle = |B\rangle \tag{S7.25}$$

as the form

$$\begin{pmatrix} I & & & & \\ -iHh & I & & & \\ & \ddots & \ddots & & \\ & & -iHh & I & \\ & & & -iHh & I \end{pmatrix} \begin{pmatrix} \psi(t_0) \\ \psi(t_1) \\ \vdots \\ \psi(t_{N_t-1}) \\ \psi(t_{N_t}) \end{pmatrix} = \begin{pmatrix} |\psi(0))\rangle \\ 0 \\ \vdots \\ 0 \\ 0 \end{pmatrix}. \tag{S7.26}$$

We can perform the quantum linear ODE solvers such as [12, Theorem 2] to produce the history state

$$|\Psi\rangle = \frac{1}{\sqrt{N_t+1}} \sum_{k=0}^{N_t} |k\rangle|\psi(t_k)\rangle \tag{S7.27}$$

with query and gate complexity

$$\mathcal{O}(Q) \tag{S7.28}$$

as defined in Theorem S7.1. Here we use the fact that the rescaling factor of the Hamiltonian dynamic satisfies $g = \frac{\max_{t\in[0,T]} \|\Psi(t)\|}{\|\Psi(T)\|} = 1$, so there are no additional factors.

The quantum linear ODE solver requires $\mathcal{O}(Q)$ copies of the input states $|\psi(0))\rangle$ in the linear system (S7.25), while the Hamiltonian simulation algorithm only requires a single copy of $|\psi(0))\rangle$. We state the results as below.

**Problem 3.** *We consider the harmonic oscillator system (S7.3) or (S7.14). Under the same assumption of Problem 2, and given certain quadrature nodes $0 = t_0 < t_1 < \ldots < t_{N_t} = T$, the goal is to produce the history state*

$$|\Psi\rangle = \frac{1}{\sqrt{N_t+1}} \sum_{k=0}^{N_t} |k\rangle|\psi(t_k)\rangle, \tag{S7.29}$$

*within $\ell_2$ error tolerance $\epsilon$.*

**Theorem S7.3.** *Problem 3 can be solved with a quantum algorithm that makes*

$$\mathcal{O}\Big(q\sqrt{\kappa_A}T\,\mathrm{polylog}(1/\epsilon)\Big) \tag{S7.30}$$

*queries to the unitaries $U_M$ and $U_F$ that prepare $M$ and $F$, and the unitaries $U_I$ and $U_b$ that prepare $\boldsymbol{x}(0)$ and $\boldsymbol{b}(t)$, where $\kappa_A = \frac{K_{\max}}{m_{\min}}$, $m_{\min} \geqslant m_j \geqslant m_{\min} > 0$, and $K_{\max} \geqslant K_{jk}$, $q = \frac{\|\boldsymbol{x}_0\|+\|\boldsymbol{b}\|_{L^1}}{\|\boldsymbol{x}(T)\|}$, and $\|\boldsymbol{b}\|_{L^1} = \int_0^T \boldsymbol{b}(s)ds$. The one- or two-qubit gate complexity is larger by a poly-logarithmic factor.*

## S7.4 Quantum algorithms for simulating Langevin dynamics

For molecular dynamics with stochastic effects, we consider the Langevin dynamics (S2.16) as the problem model

$$M\frac{\mathrm{d}^2\boldsymbol{u}}{\mathrm{d}t^2}+\gamma\frac{\mathrm{d}\boldsymbol{u}}{\mathrm{d}t}+K\boldsymbol{u}+\sigma\xi(t)=0. \tag{S7.31}$$

Here $\gamma>0$ is the friction coefficient from the interaction of the protein with the surrounding solvent. In addition, $\xi(t)$ is a white noise with independent entries acting on each velocity component. The noise amplitude is related to the damping coefficient according to the fluctuation-dissipation theorem,

$$\sigma=\sqrt{2k_BT\gamma}.$$

To formulate an efficient quantum algorithm for (S7.31), we first show that the Langevin equation (S7.31) can be converted into a stochastic Schrödinger equation. Again motivated by [19], we introduce variable $\boldsymbol{v}(t)$, and consider the following dynamics,

$$\frac{d}{dt}\begin{bmatrix}\boldsymbol{u}\\ \boldsymbol{v}\end{bmatrix}=-i\begin{bmatrix}0 & B\\ B^\dagger & 0\end{bmatrix}\begin{bmatrix}\boldsymbol{u}\\ \boldsymbol{v}\end{bmatrix}-\begin{bmatrix}0 & 0\\ 0 & \gamma I\end{bmatrix}\begin{bmatrix}\boldsymbol{u}\\ \boldsymbol{v}\end{bmatrix}+\begin{bmatrix}0\\ \sigma I\end{bmatrix}\xi(t) \tag{S7.32}$$

By differentiating the first equation, followed by a substitution of the second equation, we obtain the Langevin dynamics,

$$\frac{d^2}{dt^2}\boldsymbol{u}=-BB^\dagger\boldsymbol{u}-\gamma\frac{d}{dt}\boldsymbol{u}+\sigma\xi(t). \tag{S7.33}$$

Therefore, by choosing $B$, such that $K=BB^\dagger$, we can map the Langevin equation (S7.31) to a stochastic Schrödinger equation. However, it is interesting to note that, unlike the stochastic Schrödinger equation from the theory of open quantum systems [15], this equation has an additive noise, instead of a multiplicative noise.

We will express (S7.32) as a stochastic differential equation in the Itô's form,

$$\frac{d}{dt}\left|\phi\right\rangle=-(iH+\gamma I)\left|\phi\right\rangle+\Sigma\xi(t). \tag{S7.34}$$

Here $H$ is defined as (S7.19) with $\|H\|=\sqrt{\kappa_A}$, and $\Sigma$ is a matrix with the property that

$$\Sigma\Sigma^T=\begin{bmatrix}0 & 0\\ 0 & \sigma^2 I\end{bmatrix}. \tag{S7.35}$$

Define an operator $\rho(t):=\mathbb{E}[|\phi(t)\rangle\langle\phi(t)|]$. Then the Itô Lemma implies that $\rho$ solves the following master equation,

$$\frac{d}{dt}\rho=-i[H,\rho]-\{\gamma I,\rho\}+\Sigma\Sigma^\dagger, \tag{S7.36}$$

where $\gamma<0$.

In the Langevin dynamics model, we are interested in solving the following problem.

**Problem 4.** *We consider the Langevin dynamics (S7.36). Under the same assumption of Problem 1, the goal is to produce $\rho$ within $\ell_2$ error tolerance $\epsilon$.*

**Theorem S7.4.** *Problem 4 can be solved using*

$$\mathcal{O}\Big(\sqrt{\kappa_A}T + \log(1/\epsilon)\Big) \tag{S7.37}$$

*queries to unitaries $U_M$ and $U_F$ that prepare $M$ and $F$ and the unitaries $U_I$ for $\rho(0)$ and $\xi(t)$. The one- or two-qubit gate complexity is larger by a poly-logarithmic factor.*

*Proof.* Defined $J = -iH - \gamma I$. Then at each step, the density operator can be updated as follows,

$$\rho(t) = e^{tJ}\rho(0)e^{tJ^\dagger} + \int_0^t e^{\tau J}\Sigma\Sigma^\dagger e^{\tau J^\dagger}\mathrm{d}\tau. \tag{S7.38}$$

The first term is dissipative, due to $\gamma > 0$. The second term leads to a growth of $\rho$. We expect that as $t \to \infty$, $\rho(t) \propto (BB^\dagger)^{-1}$. So it will not blow up.

In Eq. (S7.38), the trace of the first term can be bounded as

$$\mathrm{Tr}(e^{jT}\rho(0)e^{tJ^\dagger}) = \mathrm{Tr}(\rho(0)e^{t(J^\dagger+J)}) = \mathrm{Tr}(\rho(0)e^{-2\gamma tI}) = e^{-2\gamma t}\,\mathrm{Tr}(\rho(0)) = \Theta(2^n e^{-2\gamma t}), \tag{S7.39}$$

where we have assumed that we can prepare the initial state $\rho(0)$ such that its initial variance is some constant, meaning that $\mathrm{Tr}(\rho(0)) = \Theta(2^n)$. To bound the trace of the second term, observe that $\mathrm{Tr}\big(\Sigma\Sigma^\dagger\big) = \delta^2\mathrm{dim}(B) = 2^n\sigma^2$. We have

$$\mathrm{Tr}\left(\int_0^t e^{\tau J}\Sigma\Sigma^\dagger e^{\tau J^\dagger}\mathrm{d}\tau\right) = \int_0^t \mathrm{d}\tau\,\mathrm{Tr}\left(e^{jJ\tau}\Sigma\Sigma^\dagger e^{jJ^\dagger\tau}\right) \tag{S7.40}$$

$$= \int_0^t \mathrm{d}\tau\,\mathrm{Tr}\left(\Sigma\Sigma^\dagger e^{-2j\gamma I\tau}\right) \tag{S7.41}$$

$$= \frac{1-e^{-2\gamma t}}{2\gamma}\,\mathrm{Tr}\left(\Sigma\Sigma^\dagger\right) \tag{S7.42}$$

$$= \frac{1-e^{-2\gamma t}}{2\gamma}2^n\sigma^2. \tag{S7.43}$$

Since the two terms in Eq. (S7.38) are not trace-preserving, we simulate the evolution by drawing a random sample according to the traces of the two terms and then performing the simulation of either of the terms according to the sampling outcome.

Because of Eqs. (S7.39) and (S7.43), the traces are easy to estimate. To prepare the state in Eq. (S7.38), we first sample from the probability distribution proportional to the traces of the two terms, and then we either prepare the first or the second term depending on the sample outcome.

To implement the quantum completely positive map $e^{tJ}\cdot e^{tJ^\dagger}$, it suffices to implement the Kraus operator $e^{tJ}$. It is important to note that the operator $e^{tJ}$ is essentially a scaled Hamiltonian evolution because $e^{tJ} = e^{t(-iH-\gamma I)} = e^{-\gamma}e^{-iHt}$. Using the state-of-the-art Hamiltonian simulation algorithm [51], this complete positive map can be implemented with cost $(\alpha t, +\mathrm{polylog}(1/\epsilon))$, where $\alpha$ is the normalizing constant of the block-encoding of $H$, which is upper bounded by $\sqrt{\kappa_A}$. The second term in Eq. (S7.38), i.e., $\int_0^t e^{\tau J}\Sigma\Sigma^\dagger e^{\tau J^\dagger}\mathrm{d}\tau$, can be prepared in a similar way: we just randomly sample a $\tau \in [0,t]$ and then implement the completely positive map $e^{\tau J}\cdot e^{\tau J^\dagger}$ on initial state $\Sigma\Sigma^\dagger$. Finally, to prepare the initial state $\Sigma\Sigma^\dagger$, we just use two registers, where the first holds $|1\rangle\langle 1|$ and the second holds a maximally mixed state. □

Given an observable $O$, we have the following result for estimating the expectation value $\mathrm{Tr}(O\rho)$.

**Theorem S7.5.** *Let $O$ be an observable whose block-encoding has normalizing constant $\beta$ and construction cost $Q$. For every $\epsilon, \delta > 0$, there exists a quantum algorithm that products an estimate $\xi$ of $\mathrm{Tr}(\rho O)$ such that*

$$|\xi - \mathrm{Tr}(\rho O)| \leq \epsilon$$

*with probability at least $1-\delta$. This algorithm uses each of the unitaries $U_M$ and $U_F$ that prepare $M$ and $F$, the unitaries $U_I$ for $\rho(0)$ and $\xi(t)$, and the block-encoding $Q$ of $O$ a number of $\mathcal{O}(\frac{\beta}{\epsilon}\log(1/\delta))$ times.*

*Proof.* To use Lemma S1.9, we need to implement a purification of $\rho(T)$. Note that Theorem S7.4 actually produces an ensemble instead of a purification. To create a purification, we use an additional register to coherently prepare the probability distribution. Since the probability distributions as in the proof of Theorem S7.4 are integrable, this superposition can be efficiently created by [31]. Then it is straightforward to use the algorithm in Theorem S7.4 controlled by this additional register to prepare a purification of $\rho(T)$. It suffices to use precision $\epsilon$ in this step. Then use Lemma S1.9 and the statement follows. □

# S8 Computing properties of proteins

As in classical simulations, the goal of our quantum algorithms is to compute certain properties of proteins within a given error tolerance $\epsilon$. We consider a Hamiltonian system to represent the protein system with Hamiltonian $H$. In our paper, we consider two types of input models:
(a) block encoding (BE) model: let $U$ be an $\alpha$-block-encoding of the Hamiltonian $H$;
(b) Quantum evolution (QE) model: there is a quantum algorithm $U(t)$ that prepares an amplitude-encoded solution $|\psi(t)\rangle$ at time $t$.

We consider properties that can be expressed through an observable $O$. We let $V$ be an $\beta$-block-encoding of the observable $O$.

The quantum evolution (QE) model is inspired by the Hamiltonian evolution model [24], where we have the explicit operator $U = e^{\mathrm{i}Ht}$. The QE models contain the quantum simulation of the homogeneous harmonic oscillator system (Problem 1), and the QE model can also include other dynamical models, such as the inhomogeneous oscillator system (Problem 2), history-state model (Problem 3), and Langevin dynamical system (Problem 4).

We discuss various types of application models with queries to the input model of $H$ and $O$ in the following sections.

## S8.1 Kinetic and potential energy

Inspired by [48, 8, 50], we first estimate the kinetic and potential energy of protein molecules.

**Theorem S8.1** (Theorem 5,6 of [8]). *Given a unitary $U_D$ for a subset of molecules $D \subset [n]$, s.t. $U_D|j\rangle = -|j\rangle$ for $j \in D$ and $U_D|j\rangle = |j\rangle$ for $j \notin D$. Let $E$ be the total energy, which is conserved in time, $K_D(t) = \frac{1}{2}\sum_{j\in V} m_j \dot{x}_j^2(t)$ be the kinetic energy, and $P_D(t) = \frac{1}{2}\sum_{(j,j)\in V} \kappa_{jj} x_j^2(t) + \frac{1}{2}\sum_{(j,k)\in V} \kappa_{jk}(x_j(t) - x_k(t))^2$ be the potential energy. Then*
*(i) a quantum algorithm can produce $\hat{k}_D(t)$ such that*

$$\left|\hat{k}_D(t) - K_D(t)/E\right| < \epsilon \tag{S8.1}$$

*with probability $1-\delta$, which makes $\mathcal{O}\left(\frac{\log(1/\delta)}{\epsilon}\right)$ queries of $U_D$ and Hamiltonian simulation algorithm $U(t)$ that prepares $|\psi(t)\rangle$ in Theorem S7.1.*
*(ii) a quantum algorithm can produce $\hat{p}_D(t)$ such that*

$$\left|\hat{p}_D(t) - P_D(t)/E\right| < \epsilon, \tag{S8.2}$$

*with probability $1-\delta$, which makes $\mathcal{O}\left(\frac{\log(1/\delta)}{\epsilon}\right)$ queries of $U_D$ and Hamiltonian simulation algorithm $U(t)$ that prepares $|\psi(t)\rangle$ in Theorem S7.1.*

Similar as Proof of Theorem 5 of [8], we note that $K_D(t)/E = \langle\psi(t)|\mathcal{P}|\psi(t)\rangle$ with projection $\mathcal{P} = (I - U_D)/2$. We can use amplitude estimation to estimate $\langle\psi(t)|U_D|\psi(t)\rangle$ within $2\epsilon$ and success probability $1-\delta$ with $\mathcal{O}(\frac{\log(1/\delta)}{\epsilon})$ use of $U_D$ and copies of $|\psi(t)\rangle$, which is produced by $U(t)$.

We are also interested in producing dense outputs (time-accumulated observables) from the protein dynamics [48, 50]. For the general quantum dense output problem with its early fault-tolerant quantum algorithm and nearly optimal time quantum algorithm, we refer to Problem 1 and Table 1 of [50].

As a certain type of dense output, we consider the time-accumulated kinetic energy of protein molecules, denoted as $K_V$. This quantity is closely related to time series analysis and spectral analysis of molecular dynamics, and it is of importance in understanding the effects of molecular aggregates and polymers. We follow the procedure in Section 6 of [48]: given the total energy $E_T = ET$ and discrete time subinterval $\mathcal{D}_T = \{t_0 = 0, t_1, \ldots, t_{K-1}, t_K = T\}$, the ratio of kinetic energy $K_V/E_T = \langle\psi|\mathcal{O}|\psi\rangle$ associates with the observable $\mathcal{O}$ related to $\mathcal{D}_T$ and the history state $|\psi\rangle = \frac{1}{\sqrt{K+1}}\sum_{k=0}^{K}|k\rangle|\psi(t_k)\rangle$.

**Theorem S8.2.** *Given a unitary $U_D$ for subset of molecules and time $D \subset [n] \times \mathcal{D}_T$, $\mathcal{D}_T = \{t_0 = 0, t_1, \ldots, t_{K-1}, t_K = T\}$, s.t. $U_D|j,k\rangle = -|j,k\rangle$ for $(j,k) \in D$ and $U_D|j,k\rangle = |j,k\rangle$ for $(j,k) \notin D$. Let $E_T = ET$, $E$ be the total energy preserved in time, and $K_V = \frac{1}{2}\sum_{(j,k)\in V} m_j \dot{x}_j^2(t_k)$ be the time-accumulated kinetic energy. Then a quantum algorithm can produce $\hat{k}_V$ such that*

$$|\hat{k}_V - K_V/E_T| < \epsilon \tag{S8.3}$$

*with probability $1-\delta$, which makes $\mathcal{O}(\frac{\log(1/\delta)}{\epsilon})$ queries of $U_D$ and quantum linear ODE solver $U(t)$ that prepares the history state $|\psi\rangle = \frac{1}{\sqrt{K+1}}\sum_{k=0}^{K}||k\rangle\psi(t_k)\rangle$ in Theorem S7.3.*

## S8.2 Low vibration modes

In the context of protein dynamics, the eigenvector of the lowest nonzero eigenvalue are often associated with the structural changes, and more importantly, the protein functions [10]. The main observation is that atomic displacements along high-frequency modes are energetically less favorable than those of equal magnitude along low-frequency modes.

Due to the translation symmetry, the stiffness matrix has a trivial null space. For example, the matrix that determines the vibration modes (e.g., see Eq. (S2.10)) has one zero eigenvalue with eigenvector, $N^{-1/2}(1, 1, \cdots, 1)$. Similarly the matrix (e.g., (S2.13)) has three zero eigenvalues with zero eigenvectors,

$$N^{-1/2}(1, 0, 0, 1, 0, 0, \cdots, 1, 0, 0), N^{-1/2}(0, 1, 0, 0, 1, 0, \cdots, 0, 1, 0), N^{-1/2}(0, 0, 1, 0, 0, 1, \cdots, 0, 0, 1).$$

Similarly, rotational invariance induces another three-dimensional null space. We denote the null space (or eigenspace with the 6 zero eigenvalues) by $Y$. Therefore, according to the Courant-Fischer Theorem, the problem of finding the lowest normal mode can be formulated as follows,

$$\min_{\boldsymbol{v}\in Y^\perp} \frac{\boldsymbol{v}^T H \boldsymbol{v}}{\boldsymbol{v}^T \boldsymbol{v}} = \min_{|\psi\rangle \in Y^\perp} \langle\psi| H |\psi\rangle. \tag{S8.4}$$

For this purpose of estimating low modes, we need a unitary

$$U(t) = \exp(-itH),$$

and an initial state $|\psi_0\rangle$ that has enough overlap with $|\psi\rangle$ .

Given known zero eigenspace $Y$ and nonzero spectral gap $\Delta$, we construct a projector $P_{Y^\perp} = I - \sum_{\boldsymbol{v}\in Y^\perp} \boldsymbol{v}\boldsymbol{v}^T$ onto nonzero eigenspace $Y^\perp$. Given initial state $|\psi_0\rangle$ that has overlap with $|\psi\rangle$ as $p_0 = |\langle\psi_0|\psi\rangle|^2$, if there is a $(\alpha, a, \epsilon)$-block-encoding of $H$, we can perform quantum eigenstate filtering to estimate the (nonzero) ground state with cost $\mathcal{O}\big(\alpha/(\Delta\sqrt{p_0}\epsilon)\big)$ [46, Theorem 6].

To ensure that the initial state $|\psi_0\rangle$ has sufficient overlap with $|\psi\rangle$, we may select a vector $|\psi_0\rangle$ from a subspace generated from rotation-translation blocks (RTB) [26]. Such a subspace consists of atomic configurations where the atoms within each residue follow a rigid body rotation and translation, it has been demonstrated to be a very effective approximation of the low eigenmodes of an all-atom model [42, 20]. In this case, the total Hessian matrix is projected to a much smaller matrix [20],

$$H_{\text{proj}} = B^T H B,$$

where $B \in \mathbb{R}^{N\times 6n} = [b_1, b_2, \cdots, b_{6n}]$ is an orthogonal matrix (the number of atoms $N \gg$ the number of blocks $6n$), with each column representing a rotational or translational mode of a residue. The orthogonal matrix $B$ is given by [42, 20]

$$B^\mu_{J,j_\nu} = \begin{cases} \sqrt{\frac{m_j}{M_j}}\delta_{\mu\nu}, & \mu = 1, 2, 3; \\ \sum_{\alpha,\beta} I_{J_{\mu-3,\alpha}}^{-1/2} \sqrt{m_j}(r_j - r_J^0)_\beta \epsilon_{\alpha\beta\nu}, & \mu = 4, 5, 6. \end{cases} \tag{S8.5}$$

Here $J$ and $j$ subscript label blocks and atoms, $\mu = 1, 2, 3$ and $\mu = 4, 5, 6$ label translations and rotations, $m_j$ and $r_j$ label the mass and Cartesian coordinates of the atom $j$, $M_J$, $I_J$, and $r_J^0$ label the total mass, moment of inertia, and center of mass of the block $J$, $\delta$ is the Kronecker delta, and $\epsilon$ is the permutation over $\alpha, \beta, \nu$ over $\{1, 2, 3\}$.

The low-eigen modes of $H_{\text{proj}}$, due to the much smaller dimension, can be computed with classical algorithms. For example, let $\boldsymbol{w}$ be an eigenvector of $H_{\text{proj}}$. Then, we can choose,

$$|\psi_0\rangle = w_1 |b_1\rangle + w_2 |b_2\rangle + \cdots + w_{6n} |b_{6n}\rangle .$$

The RTB approach has been demonstrated to be quite effective in approximating low eigenmodes [57, 42]. One way to quickly check whether the overlap between $|\psi_0\rangle$ and $|\psi\rangle$ is to compute the residual error. Consider $E = \langle\psi_0| H |\psi_0\rangle$, which is known as the Ritz value. Then

$$|\langle\psi_0|\psi\rangle|^2 \geq 1 - \frac{\|H\psi_0 - E\psi_0\|^2}{\Delta^2}, \tag{S8.6}$$

here $\Delta$ refers to the spectral gap and the numerator is the residue error, which can be directly examined.

Overall, the RTB approach relies on a partition of the protein into more rigid structures to capture the low-lying eigenmodes. In addition to this natural choice of residues, one can also use other partition schemes, e.g, based on atomic density [20] or rigidity analysis [39].

Given an initial good guess $|\psi_0\rangle$ as prepared above, we can filter out zero eigenstates by the projector $P_{Y^\perp} = I - \sum_{\boldsymbol{v} \in Y^\perp} \boldsymbol{v}\boldsymbol{v}^T$, and then prepare the filtered initial state

$$|\psi_0'\rangle = \frac{P_{Y^\perp} |\psi_0\rangle}{\sqrt{P_{Y^\perp} |\psi_0\rangle}}.$$

The state $|\psi_0'\rangle$ has zero overlap with the zero eigenspace $Y$, and has $p_0$ overlap with the nonzero eigenstate $|\psi\rangle = |\psi_6\rangle$, where $|\langle\psi_0|\psi\rangle|^2 = p_0 \geqslant \gamma^2$. We then use this state to prepare the first nonzero eigenvalue and eigenstate.

Lin and Tong developed LCU-based quantum eigenstate filtering method for the ground state preparation and energy estimation with near-optimal cost [46].

For the purpose of early fault-tolerant quantum algorithms, we can employ the QET-U approach, a modified QSP approach with a shorter quantum circuit.

**Theorem S8.3** (Theorem 11 of [24])**.** *Suppose we are given a Hamiltonian $H$ on $n$-qubit whose spectrum is contained in $[\eta, \pi - \eta]$, for $\eta > 0$. Given the Hamiltonian evolution input $U_H = e^{-iH}$. Also suppose we have an initial state $|\psi_0\rangle$ prepared by circuit $U_I$, with lower bound for the overlap: $|\langle\psi_0|\psi\rangle|^2 = p_0 \geqslant \gamma^2$. Then the ground state energy can be prepared to precision $\epsilon$ with probability $1 - \delta$ with the following cost:*

*(i) $\mathcal{O}\Big(\frac{1}{\gamma\epsilon}\log(1/\delta)\Big)$ queries to (controlled-)$U_H$ and $\mathcal{O}\Big(\frac{1}{\gamma}\log(1/\delta)\Big)$ queries to $U_I$;*

*(ii) three ancilla qubits;*

*(iii) $\mathcal{O}\Big(\frac{1}{n\gamma}\log(1/(\delta\epsilon)) + \frac{1}{\gamma\epsilon}\log(1/\delta)\Big)$ number of other one- or two-qubit gates;*

*(iv) $\mathcal{O}\Big(\frac{1}{\gamma\epsilon}\log(1/\delta)\Big)$ query depth of $U_H$.*

For large overlap $\gamma = \Omega(1)$, we can employ a simple quantum circuit with classical post-processing procedure. The algorithm samples from Hadamard tests, and uses the samples to approximately reconstruct the cumulative distribution function (CDF) of the spectral measure associated with the Hamiltonian, and then estimate the ground state energy with high confidence.

Let the initial state be expanded as $|\psi_0\rangle = \sum_k \alpha_k |\psi_k\rangle$ in the eigenbasis of $H$, and let $p_k = |\alpha_k|^2$ be the overlap with the $k$-th eigenstate. They considered the spectral density function $p(x) = \sum_k p_k \delta(x - \lambda_k)$ and its cumulative distribution function (CDF) $C(x) = \int_x p(x)\mathrm{d}x$. The algorithm in [47] aims to estimate $\lambda_0$ by locating the first nonzero point of $C(x)$. In our case, when we choose $|\phi_0'\rangle = \frac{P_{Y^\perp}|\psi_0\rangle}{\sqrt{P_{Y^\perp}|\psi_0\rangle}}$, we observe that $p_0 = p_1 = \cdots = p_5 = 0$. So we can straightforwardly perform the quantum eigenvalue estimation algorithm in [47] to estimate $\lambda_6$.

**Theorem S8.4** (Corollary 3 of [47]). *Suppose we have an initial state $|\psi_0\rangle$ prepared by circuit $U_I$, with lower bound for the overlap: $|\langle\psi_0|\psi\rangle|^2 = p_0 \geqslant \gamma^2$. There is a quantum algorithm that estimates the ground state energy and prepares the ground state to precision $\epsilon$ with probability $1-\delta$ with the following cost*

*(i)* $\mathcal{O}\Big(\frac{1}{\gamma^4\epsilon}\log(1/\delta)\Big)$ *queries to (controlled-)*$U_H$ *and* $\mathcal{O}\Big(\frac{1}{\gamma^4}\log(1/\delta)\Big)$ *queries to* $U_I$*;*

*(ii)* $\mathcal{O}(1)$ *ancilla qubits;*

*(iii)* $\mathcal{O}\Big(\frac{1}{\gamma^4\epsilon}\log(1/\delta)\Big)$ *number of other one- or two-qubit gates;*

*(iv)* $\mathcal{O}\Big(\frac{1}{\epsilon}\log\Big(\frac{1}{\gamma\nu}\Big)\Big)$ *query depth of* $U_H$*;*

*and classical post-processing cost* $\mathcal{O}\Big(\frac{1}{p_0^2}\,\mathrm{polylog}(\frac{1}{p_0\epsilon})\Big)$.

For example, the approaches in [27, 45] usually extract multiple normal modes as a starting point to study the actual dynamics of proteins.

We may investigate other early fault-tolerant quantum algorithms, such as QET-U [24], QCELS [21, 22], and RPE [52, 43]. But if we aim to estimate multiple eigenstates and eigenvalues, we intend to employ MM-QCELS [22] and RMPE [43].

## S8.3 Density of States and Chebyshev moments

Here we discuss the estimation of the density of states (DoS), given by,

$$\varrho(\lambda) = \frac{1}{N}\sum_{j=0}^{N-1}\delta(\lambda-\lambda_j), \tag{S8.7}$$

for the eigenvalue distribution of the adjacency matrix of the protein network [38]. Specifically, $\{\lambda_j\}$ are eigenvalues of the Hamiltonian $H$, associated with eigenvectors $\{|\psi_j\rangle\}$. We are given an $\alpha$-block-encoding of $H$. More generally, we can estimate the local density of the state

$$\varrho_{\vec{r}}(\lambda) = \frac{1}{N}\sum_{j=0}^{N-1}\delta(\lambda-\lambda_j)|\langle\psi_j|\vec{r}\rangle|^2. \tag{S8.8}$$

Notice that the density of states (S8.7) can be obtained from the local density of states by integration over $\vec{r}$.

In general, we can consider a function $f(\lambda)$ defined via an observable $A$

$$f(\lambda) = \sum_{j=0}^{N-1} \delta(\lambda - \lambda_j) \langle \psi_j | A | \psi_j \rangle. \tag{S8.9}$$

We approach this problem by computing the integral of $f$ over an interval $[a, b]$, specifically, the moments of a Chebyshev expansion of $f(\lambda)$, as we show below. Following [54], there exists a polynomial $w(x)$ that has degree $d = \mathcal{O}(\frac{f_{\max}}{\epsilon} \log \frac{f_{\max}}{\epsilon})$ and satisfies $|w(x)| \leqslant 1$, such that

$$\begin{aligned} \int_a^b f(\lambda) \mathrm{d}\lambda \approx \alpha \int_{-1}^{1} f(\alpha x) w(x) \mathrm{d}x &= \int_{-1}^{1} \sum_{j=0}^{N-1} \delta(\alpha x - \lambda_j) \langle \psi_j | A | \psi_j \rangle w(x) \mathrm{d}x \\ &= \mathrm{Tr}\Big( A \sum_{j=0}^{N-1} \int_{-1}^{1} \delta(x - \lambda_j/\alpha) w(x) |\psi_j\rangle\langle\psi_j| \Big) \\ &= \mathrm{Tr}\Big( A \sum_{j=0}^{N-1} w(\lambda_j/\alpha) |\psi_j\rangle\langle\psi_j| \Big) = \mathrm{Tr}\Big( A w(H/\alpha) \Big). \end{aligned} \tag{S8.10}$$

We then calculate the moments of $f(\lambda)$ based on Chebyshev polynomial of the first kind $T_k(x)$

$$\mu_k^f = \int_a^b T_k(x) f(\alpha x) \mathrm{d}x, \tag{S8.11}$$

and from the calculations above, we find,

$$\mu_k^f \approx \mathrm{Tr}\Big( A T_k(H/\alpha) \Big). \tag{S8.12}$$

To compute the density of state $\rho(\lambda)$ (S8.7), we choose $A = I/N$ in $f(\lambda)$, such that

$$\int_a^b \varrho(\lambda) \mathrm{d}\lambda \approx \mathrm{Tr}\Big( \frac{I}{N} w(H/\alpha) \Big), \tag{S8.13}$$

$$\mu_k^{\varrho} \approx \mathrm{Tr}\Big( \frac{I}{N} T_k(H/\alpha) \Big). \tag{S8.14}$$

The observable estimation lemma [54] is stated as below.

**Lemma S8.5** (Lemma 5 of [54])**.** *Let $U_A$ be an $\alpha$-block-encoding of the Hermitian matrix $A$ and $U_A$ can be implemented with $Q$ elementary gates. Let $U_I$ prepare $\rho$ with $R$ elementary gates. For $\epsilon > 0$, there is a quantum algorithm that estimates $\mathrm{Tr}(A\rho)$ within $\epsilon$ with probability $\Omega(1)$ with gate complexity $\mathcal{O}((R+Q)\frac{\alpha}{\epsilon})$.*

Given a $\alpha$-block-encoding of the Hermitian $A$, there is a $(\alpha d)$-block-encoding of $f(A)$, where $f$ is a $d$-degree polynomial. We use the lemma below to present the complexity results.

**Theorem S8.6** (Theorem 11 of [54])**.** *Let $U_H$ be an $\alpha$-block-encoding of the Hermitian $H$. For any $\epsilon, \delta > 0$:*

*1. There exists a quantum algorithm that estimates $\int_a^b \varrho(\lambda) \mathrm{d}\lambda$ with $\mathcal{O}(\frac{\alpha \varrho_{\max}}{\epsilon^2})$ queries to $U_H$ and*

*overall quantum gate complexity* $\mathcal{O}\Big((\frac{\alpha\varrho_{\max}}{\epsilon}+\log N)\cdot\frac{\log(1/\delta)}{\epsilon}\Big)$ *and classical pre-processing* $\mathcal{O}(\mathrm{poly}(\frac{\varrho_{\max}}{\epsilon}))$, *where* $\varrho_{\max}$ *is an upper bound of the dimension of the largest eigenspace of* $H$.
*2. There exists a quantum algorithm that estimates* $\mu_k^\varrho$ *with* $\mathcal{O}(\frac{\alpha n}{\epsilon})$ *queries to* $U_H$ *and overall quantum gate complexity* $\mathcal{O}\Big((\alpha k+\log N)\cdot\frac{\log(1/\delta)}{\epsilon}\Big)$, *where* $k$ *is the degree of Chebyshev polynomial.*

The above algorithm can be extended to the local density of states in Eq. (S8.8). This can come up when we are working with a Hamiltonian describing a single particle in real space or some space with a notion of locality. For every position $\vec{r}$, there is a state $|\psi(\vec{r})\rangle$ denoting the state with the particle at $\vec{r}$. The algorithms for estimating the LDOS are a simple modification of the algorithms for DOS: instead of preparing a maximally mixed state we simply prepare $|\psi(\vec{r})\rangle$. If $|\psi(\vec{r})\rangle$ has a $O(R)$ preparation unitary, the new circuit complexities are the same as those in Theorem S8.6 but with $\log D$ replaced with $R$.

An alternative definition of the local density of the state is given by

$$\varrho_{\vec{r}}(\lambda)=\frac{1}{N}\sum_{j=0}^{N-1}\delta(\lambda-\lambda_j)||\psi_j(\vec{r})\rangle|^2. \tag{S8.15}$$

The contribution of each state is weighted by the density of its wave function at the point $\vec{r}$. We can further generalize the local density of states further to

$$\varrho_{\vec{r},\vec{r}'}(\lambda)=\frac{1}{N}\sum_{j=0}^{N-1}\delta(\lambda-\lambda_j)|\langle\psi_j(\vec{r})|\psi_j(\vec{r}')\rangle|^2. \tag{S8.16}$$

This is called the spectral function and it is a function with each wave function evaluated as a different position. It can be interpreted as a Green's function. This type of function can also be treated using a similar quantum algorithm.

## S8.4 Correlation and root mean square of displacement

In this section, we develop quantum algorithms for estimating the cross-correlation and root mean square of the atomic displacement based on the block-encoding of the pseudo-inverse of the Hamiltonian.

Let $\omega_k^2$ be the $k$th eigenvalue of $H$ with eigenvector $\boldsymbol{v}_k$. Then $H$ admits the following spectral decomposition,

$$H=\sum_{k=7}^{3N}\omega_k^2\boldsymbol{v}_k\boldsymbol{v}_k^T. \tag{S8.17}$$

Recall that the first six eigenvalues of $H$ are zero. Therefore, the pseudo-inverse is given by,

$$H^-=\sum_{k=7}^{3N}\frac{1}{\omega_k^2}\boldsymbol{v}_k\boldsymbol{v}_k^T. \tag{S8.18}$$

We can efficiently block encode the (pseudo) inverse of Hamiltonian $H$. According to [55, 29, 56], we have the following result.

**Lemma S8.7** (Proposition 9 of [56]). *Let $H$ be a Hermitian matrix that its eigenvalues is on $[-\alpha, -1/\beta] \cup [1/\beta, \alpha]$, with condition number $\kappa = \alpha\beta$. Given $U_H$ that is a $(\alpha, a, \epsilon)$-block-encoding of $H$, we can implement $U^-$ that is a $(\beta', a+2, \epsilon')$-block-encoding of $H^-$ with $\beta' = \frac{16}{3}\beta$, $\epsilon' = 4d(\sqrt{\frac{\epsilon}{\alpha}} + \delta)\beta'$, which consists of $\mathcal{O}(d)$ uses of $U_H$ and $\mathcal{O}((a+1)d)$ uses of additional one- or two-qubit gates, where $d = \mathcal{O}(\kappa \log(1/\delta))$.*

Given the block-encoded (inverse) Hamiltonian, we can use amplitude estimation to estimate the expectation of block-encoded observables.

Based on the observable estimation lemma as in Lemma S8.5, we have $\alpha = 1/\beta$, and $Q = \mathcal{O}(d) = \mathcal{O}(\kappa \log(1/\delta))$. Therefore, we can estimate $\mathrm{Tr}(H^-\rho)$ for certain observable $\rho$ with gate complexity $\mathcal{O}((R+d)\frac{1}{\beta\epsilon}) = \mathcal{O}(\frac{R}{\beta\epsilon} + \frac{\alpha}{\epsilon}\log(1/\delta))$.

Meanwhile, often of interest is the cross-correlation of the atomic displacement, i.e.,

$$\mathbb{E}[\boldsymbol{u}_i \boldsymbol{u}_j]. \tag{S8.19}$$

One can show that the cross-correlation can be expressed in terms of the matrix inverse,

$$\mathbb{E}[\boldsymbol{u}_i \boldsymbol{u}_j] = H^-_{ij} = \mathrm{Tr}\big(H^- |j\rangle \langle i|\big). \tag{S8.20}$$

Therefore, we can perform the observable estimation with $\rho = |j\rangle\langle i|$. Although the probability of measuring a single index $|j\rangle\langle i|$ is small (i.e. it is highly likely to return the zero result), we can estimate a collection of indices $\rho = \sum_{(i,j)\in\mathcal{I}} |j\rangle\langle i|$.

Another important statistical quantity is the root mean square displacement [23]. which is related to the eigenvalues as follows,

$$\mathrm{RMSE} = \sqrt{\frac{1}{N}\sum_j \mathbb{E}[\boldsymbol{u}_i^2]} = \sqrt{\frac{1}{N}\sum_k \frac{1}{\omega_k^2}}. \tag{S8.21}$$

We can perform amplitude estimation to produce $\mathrm{Tr}(H^-\rho)$ with $\rho = I$.

We summarize the results as follows.

**Theorem S8.8.** *Let $U_H$ be an $\alpha$-block-encoding of the Hermitian $H$ and $U_H$ can be implemented with $R$ elementary gates. Let $U_I$ prepare $\rho = \sum_{(i,j)\in\mathcal{I}} |j\rangle\langle i|$ with $R$ elementary gates. For any $\epsilon > 0$:*

*1. There exists a quantum algorithm that estimates the cross-correlation of displacement $\sum_{(i,j)\in\mathcal{I}} \mathbb{E}[\Delta R_i \Delta R_j]$ within $\epsilon$, with gate complexity $\mathcal{O}\Big(\frac{R}{\beta\epsilon} + \frac{\alpha}{\epsilon}\Big)$.*

*2. There exists a quantum algorithm that estimates the root mean square of displacement $\sqrt{\frac{1}{N}\sum_j \mathbb{E}[\Delta R_i^2]}$ within $\epsilon$ with gate complexity $\mathcal{O}\Big(\frac{R}{\beta\epsilon} + \frac{\alpha}{\epsilon}\Big)$.*

### S8.5 Molecular dynamic control

We combine the optimal control theory and molecular dynamics for protein folding problems [4].

The general Linear-Quadratic-Regulator (LQR) problems can be formulated based on a driven ODE,

$$\frac{d}{dt}\boldsymbol{x}(t) = A\boldsymbol{x}(t) + B\boldsymbol{u}(t). \tag{S8.22}$$

For the molecular dynamical control, the course-grained folding dynamics is governed by the equation of motion

$$M\frac{\mathrm{d}^2\boldsymbol{u}(t)}{\mathrm{d}t^2}+\gamma\frac{\mathrm{d}\boldsymbol{u}(t)}{\mathrm{d}t}+K\boldsymbol{u}(t)=\boldsymbol{f}(t). \tag{S8.23}$$

Here $M$ is the mass, $\gamma$ is the friction, $K$ is the connectivity matrix, and $F$ is the $n$-dimensional force field. For instance, we have access to control $F$ with a low dimensional input $u=[u_1,\dots,u_m]^T$ ($m \ll n$), such that $u(t)=\sum_{j=1}^m u_j(t)e_j$, where $e_j$ is a fixed vector. Here we can reformulate the equation of motion as the ODE with new variable $\boldsymbol{x}(t)=[R(t),\dot{R}(t)]$.

In addition, the cost function can be defined either over an infinite horizon ($T=+\infty$) or a finite horizon. In the latter case, the cost function is defined as,

$$J[\boldsymbol{f}]=\frac{1}{2}\boldsymbol{u}(T)^T S\boldsymbol{u}(T)+\int_0^T \boldsymbol{u}(t)^T Q\boldsymbol{u}(t)+\boldsymbol{f}(t)^T R\boldsymbol{f}(t)dt. \tag{S8.24}$$

A convenient framework for computing the gradient of $J$ with respect to the control variable is the Lagrange multiplier approach [41, Part IV], which expresses the gradient through an adjoint equation,

$$\frac{d}{dt}\boldsymbol{y}(t)=A\boldsymbol{y}(t)-Q\boldsymbol{x}(t),\quad \boldsymbol{y}(T)=S\boldsymbol{x}(T). \tag{S8.25}$$

Notice that this equation has to be solved backward in time using a terminal condition at time $T$. With the Lagrange multiplier, $\boldsymbol{y}(t)$, the gradient is given by,

$$\frac{\delta J}{\delta \boldsymbol{u}(t)}=R\boldsymbol{u}(t)+B^T\boldsymbol{y}(t), \tag{S8.26}$$

which can be incorporated into a gradient-based optimization algorithm, e.g., gradient descent or quasi-Newton's method [44].

**Theorem S8.9.** *For the protein dynamics (S8.23) with cost function (S8.24), let $V$ be an $\beta$-block-encoding of the observable $O$. There exists a quantum algorithm that estimates the output $J$ within $\epsilon$, with $\mathcal{O}(\frac{\beta\log(1/\delta)}{\epsilon})$ uses of $V$ and the quantum algorithm $U(t)$ that prepares $|\psi(t)\rangle$ in Theorem S7.1.*

# S9 Open Problems

Our work also indicates natural open questions for future investigation.

- Can we develop even faster quantum algorithms for certain protein problems, by employing fast-forwarded Hamiltonian simulations or quantum linear ODE solvers?
- How to prove quantum lower bounds of the quantum simulation for protein dynamics, in the sense of parameters such as the evolution time, error tolerance, and number of particles? Moreover, can we establish a solid classical lower bound for an end-to-end problem, such that there is a rigorous end-to-end exponential quantum speedup over classical algorithms?

- The current algorithms are designed to capture dynamics due to vibration modes. How to generalize the quantum algorithms for more practical molecular dynamics, e.g., ab initio molecular dynamics? In particular, can nonlinear dynamics be simulated using appropriate embedding techniques, such as Carleman or Koopman embedding [49]?
- Can we offer more practical matrix connectivity loading protocols for uploading the protein information, without utilizing circuit-based QROM?
- Can we use the initial state preparation algorithm based on rejection sampling to produce other useful quantum states with pseudo-random amplitudes?

# References


[1] J. Allcock, J. Bao, J. F. Doriguello, A. Luongo, and M. Santha. Constant-depth circuits for uniformly controlled gates and Boolean functions with application to quantum memory circuits, 2023. arXiv:2308.08539.

[2] D. An, A. M. Childs, and L. Lin. Quantum algorithm for linear non-unitary dynamics with near-optimal dependence on all parameters, 2023. arXiv:2312.03916.

[3] D. An, J.-P. Liu, and L. Lin. Linear combination of Hamiltonian simulation for nonunitary dynamics with optimal state preparation cost. *Physical Review Letters*, 131(15):150603, 2023. arXiv:2303.01029.

[4] Y. Arkun and M. Gur. Combining optimal control theory and molecular dynamics for protein folding. *PLoS One*, 7(1):e29628, 2012.

[5] S. Arunachalam, V. Gheorghiu, T. Jochym-O'Connor, M. Mosca, and P. V. Srinivasan. On the robustness of bucket brigade quantum RAM. *New Journal of Physics*, 17(12):123010, 2015. arXiv:1502.03450.

[6] N. W. Ashcroft and N. D. Mermin. *Solid state physics*. Cengage Learning, 2022.

[7] A. R. Atilgan, S. Durell, R. L. Jernigan, M. C. Demirel, O. Keskin, and I. Bahar. Anisotropy of fluctuation dynamics of proteins with an elastic network model. *Biophysical journal*, 80(1):505–515, 2001.

[8] R. Babbush, D. W. Berry, R. Kothari, R. D. Somma, and N. Wiebe. Exponential quantum speedup in simulating coupled classical oscillators. *Physical Review X*, 13(4):041041, 2023. arXiv:2303.13012.

[9] R. Babbush, C. Gidney, D. W. Berry, N. Wiebe, J. McClean, A. Paler, A. Fowler, and H. Neven. Encoding electronic spectra in quantum circuits with linear t complexity. *Physical Review X*, 8(4):041015, 2018. arXiv:1805.03662.

[10] I. Bahar, A. R. Atilgan, and B. Erman. Direct evaluation of thermal fluctuations in proteins using a single-parameter harmonic potential. *Folding and Design*, 2(3):173–181, 1997.

[11] D. Ben-Avraham. Vibrational normal-mode spectrum of globular proteins. *Physical Review B*, 47(21):14559, 1993.

[12] D. W. Berry and P. C. Costa. Quantum algorithm for time-dependent differential equations using Dyson series. *Quantum*, 8:1369, 2024. arXiv:2212.03544.

[13] D. Bluvstein, S. J. Evered, A. A. Geim, S. H. Li, H. Zhou, T. Manovitz, S. Ebadi, M. Cain, M. Kalinowski, D. Hangleiter, et al. Logical quantum processor based on reconfigurable atom arrays. *Nature*, pages 1–3, 2023. arXiv:2312.03982.

[14] G. Brassard, P. Hoyer, M. Mosca, and A. Tapp. Quantum amplitude amplification and estimation. *Contemporary Mathematics*, 305:53–74, 2002. arXiv:quant-ph/0005055.

[15] H.-P. Breuer and F. Petruccione. *The theory of open quantum systems.* Oxford University Press, USA, 2002.

[16] C. Chennubhotla and I. Bahar. Markov propagation of allosteric effects in biomolecular systems: application to groel–groes. *Molecular systems biology*, 2(1):36, 2006.

[17] C. Chennubhotla and I. Bahar. Markov methods for hierarchical coarse-graining of large protein dynamics. *Journal of computational biology*, 14(6):765–776, 2007.

[18] A. Cornelissen, Y. Hamoudi, and S. Jerbi. Near-optimal quantum algorithms for multivariate mean estimation. In *Proceedings of the 54th Annual ACM SIGACT Symposium on Theory of Computing*, pages 33–43, 2022. arXiv:2111.09787.

[19] P. C. S. Costa, S. Jordan, and A. Ostrander. Quantum algorithm for simulating the wave equation. *Physical Review A*, 99(1):012323, 2019. arXiv:1711.05394.

[20] O. N. A. Demerdash and J. C. Mitchell. Density-cluster NMA: A new protein decomposition technique for coarse-grained normal mode analysis. *Proteins: Structure, Function, and Bioinformatics*, 80(7):1766–1779, 2012.

[21] Z. Ding and L. Lin. Even shorter quantum circuit for phase estimation on early fault-tolerant quantum computers with applications to ground-state energy estimation. *PRX Quantum*, 4(2):020331, 2023. arXiv:2211.11973.

[22] Z. Ding and L. Lin. Simultaneous estimation of multiple eigenvalues with short-depth quantum circuit on early fault-tolerant quantum computers. *Quantum*, 7:1136, 2023. arXiv:2303.05714.

[23] S. E. Dobbins, V. I. Lesk, and M. J. Sternberg. Insights into protein flexibility: the relationship between normal modes and conformational change upon protein–protein docking. *Proceedings of the National Academy of Sciences*, 105(30):10390–10395, 2008.

[24] Y. Dong, L. Lin, and Y. Tong. Ground-state preparation and energy estimation on early fault-tolerant quantum computers via quantum eigenvalue transformation of unitary matrices. *PRX Quantum*, 3(4):040305, 2022. arXiv:2204.05955.

[25] P. Doruker, R. L. Jernigan, and I. Bahar. Dynamics of large proteins through hierarchical levels of coarse-grained structures. *Journal of computational chemistry*, 23(1):119–127, 2002.

[26] P. Durand, G. Trinquier, and Y.-H. Sanejouand. A new approach for determining low-frequency normal modes in macromolecules. *Biopolymers: Original Research on Biomolecules*, 34(6):759–771, 1994.

[27] J. Elezgaray and Y.-H. Sanejouand. Modal dynamics of proteins in water. *Journal of Computational Chemistry*, 21(14):1274–1282, 2000.

[28] E. Fuglebakk, N. Reuter, and K. Hinsen. Evaluation of protein elastic network models based on an analysis of collective motions. *Journal of chemical theory and computation*, 9(12):5618–5628, 2013.

[29] A. Gilyén, Y. Su, G. H. Low, and N. Wiebe. Quantum singular value transformation and beyond: exponential improvements for quantum matrix arithmetics. In *Proceedings of the 51st Annual ACM SIGACT Symposium on Theory of Computing*, pages 193–204, 2019. arXiv:1806.01838.

[30] V. Giovannetti, S. Lloyd, and L. Maccone. Quantum random access memory. *Physical review letters*, 100(16):160501, 2008. arXiv:0708.1879.

[31] L. Grover and T. Rudolph. Creating superpositions that correspond to efficiently integrable probability distributions, 2002. arXiv:quant-ph/0208112.

[32] T. Haliloglu, I. Bahar, and B. Erman. Gaussian dynamics of folded proteins. *Physical review letters*, 79(16):3090, 1997.

[33] Y. Hamoudi. Quantum sub-Gaussian mean estimator. In *29th Annual European Symposium on Algorithms (ESA 2021)*. Schloss Dagstuhl-Leibniz-Zentrum für Informatik, 2021. arXiv:2108.12172.

[34] M. Hu, S. Raj, B. Kim, W. K. Liu, S. Baik, T. Kim, B.-S. Lim, and M. K. Kim. Precise spring constant assignment in elastic network model for identification of vibration frequency and modeshape. *Journal of mechanical science and technology*, 24:1771–1780, 2010.

[35] M.-W. Hu, B. O'Riordan, B. Kim, and M. K. Kim. Comparison of all-atom and coarse-grained normal mode analysis in the elastic network model. *Journal of Mechanical Science and Technology*, 27:3267–3275, 2013.

[36] S. Izrailev, S. Stepaniants, B. Isralewitz, D. Kosztin, H. Lu, F. Molnar, W. Wriggers, and K. Schulten. Steered molecular dynamics. In *Computational Molecular Dynamics: Challenges, Methods, Ideas: Proceedings of the 2nd International Symposium on Algorithms for Macromolecular Modelling, Berlin, May 21–24, 1997*, pages 39–65. Springer, 1999.

[37] S. Jaques and A. G. Rattew. QRAM: A survey and critique, 2023. arXiv:2305.10310.

[38] C. Kamp and K. Christensen. Spectral analysis of protein-protein interactions in drosophila melanogaster. *Physical Review E*, 71(4):041911, 2005. arXiv:q-bio/0405021.

[39] K. S. Keating, S. C. Flores, M. B. Gerstein, and L. A. Kuhn. Stonehinge: hinge prediction by network analysis of individual protein structures. *Protein Science*, 18(2):359–371, 2009.

[40] I. Kerenidis and A. Prakash. Quantum recommendation systems, 2016. arXiv:1603.08675.

[41] D. E. Kirk. *Optimal control theory: an introduction.* Courier Corporation, 2004.

[42] G. Li and Q. Cui. A coarse-grained normal mode approach for macromolecules: an efficient implementation and application to Ca2+-ATPase. *Biophysical Journal*, 83(5):2457–2474, 2002.

[43] H. Li, H. Ni, and L. Ying. On low-depth quantum algorithms for robust multiple-phase estimation, 2023. arXiv:2303.08099.

[44] X. Li and C. Wang. Efficient quantum algorithms for quantum optimal control. In *International Conference on Machine Learning*, pages 19982–19994. PMLR, 2023. arXiv:2304.02613.

[45] A. N. Lima, R. J. de Oliveira, A. S. K. Braz, M. G. de Souza Costa, D. Perahia, and L. P. B. Scott. Effects of ph and aggregation in the human prion conversion into scrapie form: a study using molecular dynamics with excited normal modes. *European Biophysics Journal*, 47:583–590, 2018.

[46] L. Lin and Y. Tong. Near-optimal ground state preparation. *Quantum*, 4:372, 2020. arXiv:2002.12508.

[47] L. Lin and Y. Tong. Heisenberg-limited ground-state energy estimation for early fault-tolerant quantum computers. *PRX Quantum*, 3(1):010318, 2022. arXiv:2102.11340.

[48] J.-P. Liu, D. An, D. Fang, J. Wang, G. H. Low, and S. Jordan. Efficient quantum algorithm for nonlinear reaction–diffusion equations and energy estimation. *Communications in Mathematical Physics*, 404(2):963–1020, 2023. arXiv:2205.01141.

[49] J.-P. Liu, H. Ø. Kolden, H. K. Krovi, N. F. Loureiro, K. Trivisa, and A. M. Childs. Efficient quantum algorithm for dissipative nonlinear differential equations. *Proceedings of the National Academy of Sciences*, 118(35):e2026805118, 2021. arXiv:2011.03185.

[50] J.-P. Liu and L. Lin. Dense outputs from quantum simulations. *Journal of Computational Physics*, 514:113213, 2024. arXiv:2307.14441.

[51] G. H. Low and I. L. Chuang. Optimal Hamiltonian simulation by quantum signal processing. *Physical Review Letters*, 118(1):010501, 2017. arXiv:1606.02685.

[52] H. Ni, H. Li, and L. Ying. On low-depth algorithms for quantum phase estimation. *Quantum*, 7:1165, 2023. arXiv:2302.02454.

[53] K. Phalak, M. Alam, A. Ash-Saki, R. O. Topaloglu, and S. Ghosh. Optimization of quantum read-only memory circuits, 2022. arXiv:2204.03097.

[54] P. Rall. Quantum algorithms for estimating physical quantities using block encodings. *Physical Review A*, 102(2):022408, 2020. arXiv:2004.06832.

[55] S. Subramanian and M.-H. Hsieh. Quantum algorithm for estimating $\alpha$-renyi entropies of quantum states. *Physical Review A*, 104(2):022428, 2021. arXiv:1804.01973.

[56] S. Takahira, A. Ohashi, T. Sogabe, and T. S. Usuda. Quantum algorithms based on the block-encoding framework for matrix functions by contour integrals, 2021. arXiv:2106.08076.

[57] F. Tama, F. X. Gadea, O. Marques, and Y.-H. Sanejouand. Building-block approach for determining low-frequency normal modes of macromolecules. *Proteins: Structure, Function, and Bioinformatics*, 41(1):1–7, 2000.

[58] Y. Tong, D. An, N. Wiebe, and L. Lin. Fast inversion, preconditioned quantum linear system solvers, fast Green's-function computation, and fast evaluation of matrix functions. *Physical Review A*, 104(3):032422, 2021. arXiv:2008.13295.

[59] C. Wang and L. Wossnig. A quantum algorithm for simulating non-sparse Hamiltonians, 2018. arXiv:1803.08273.
